# Supplementary material for: Asymmetric Influence of Employees and Trading Partners on Company's Sales and its Dynamical Origin
Source: arXiv:1803.04761 source file (2018-03-13)
Supplement: Supplementary file 1 [file SI.pdf]

# SUPPLEMENTARY MATERIALS

The data employed in this study is the electronic version of COSMOS 2 database, updated yearly each January by Teikoku Databank, Ltd. This database describes over two million business firms in Japan, including two sub-databases: (1) around one million per year 'summary' firm profiles such as sales, number of employees and business type category from 1980, and (2) lists of several million trading relationships for each year since 1993. The profile of trading relationships include the direction, that is, which firm (buyer) paid to which (supplier). Only after 1993 the data fully comprehend the multi-dimensional aspect of size and growth of firms and we exclude the 1993 data in order to avoid boundary effects that might be present in 1993 trading data. The data was last updated in January, 2017. This confines our analysis to the period ending in 2015, because the 2016 sales have not been available for all the firms at the time of our study. Every firm has a unique anonymous ID. This enables tracking the firm evolution in time or in different sub-databases. A new ID can be assigned to an existing business activity by corporate reorganization such as an acquisition, a merger, and an identity change.

In order to maintain homogeneity of the included firms at the least level and time coherence between different kinds of data, we perform several steps of data compilation as follows. First, we exclude the firms that are categorized as governmental (e.g. local governments) or financial (e.g. banks and insurers) ones. This is because the definition of sales for these 'firms' is quite different from that for construction, manufacturing or wholesale firms, which are the majority of the firms in the data. By this step, we filter out possible outliers in the whole database. This procedure is applied to both sub-databases. Second, we do not use the sales data that are from a financial statement published more than 8 years before the data entry, or those without adequate timestamp. Third, we set the sales to be unknown when the end of fiscal year has changed, because some of such data is supposedly not the annual sales as the value is sometimes considerably less in the fiscal term than in previous or subsequent periods. Fourth, we determine the year to which a sale datum is assigned, according to the year in which the fiscal term ended. For example, when a firm has a fiscal year that started in April, 2000 and ended in March, 2001 like the majority of Japanese firms, sales value of the fiscal term is considered to belong to the year 2001, regardless of whether the data appeared in the database in 2002 or after. In contrast, this is not applied to employees or trading data: we always assign them to the previous year of the data entry, since the database is updated in January every year.

We directly use the raw data without normalization or adjustment for inflation. The number of trading partners of a firm is determined by counting the number of trading relations that a firm participates in the year, regardless of whether the firm is a supplier or a buyer. This amounts to computing the sum of in-degree and out-degree of every node in the directed network of trading.

Firm existence data are additionally compiled to estimate the firm exit rates. First, if any data of a firm exist for a year, the firm is considered to exist in the year. Then, when the data of a firm are not available only

for up to two consecutive years, the firm is also considered to exist in the years where the data are lacking, assuming their absence from the data is a mere consequence of accidents. Before the compilation of the existence data, the first and fourth steps of data exclusion done above for the compilation of quantitative data are also applied to assure the consistency between both datasets.

The data amount before and after the compilation is plotted in Fig. S1 against year during the 1994–2015 period. We note that the data amount is generally increasing. One can see that the number of the firms with complete data of all size variables (i.e. $k$, $l$ and $s$) is currently over 0.8 million per year after filtering. The number of existent firms is usually more than that in the sub-database of sales and employees, as the existence is assumed for some firms that only appear in the trading data or ones with temporarily missing data. Two jumps of trading data increase (2007–2008 and 2010–2011) are evident in Fig. S1b. The second jump is due to the data of trading involving financial or governmental organizations, since we see no jump in the same period after the filtering. On the other hand, the first one is the consequence of revised methods of data collection that are only related to trading relations data; trading relations which are mentioned only in on-demand reports became included in the database in 2008. Indeed, there is no comparable jump in the number of 'summary' profile data. We also note that the number of exiting or disappearing firms is quite stable compared to the number of entering firms, which implies that the former is less affected by the fluctuation of efforts paid on data collection.

All size variables are distributed in fat-tailed manners at the upper side, as shown in Fig. S2. Their distribution functions for every year are plotted in the figure, with the color gradient from blue through black to red indicating the direction from older data to newer ones. We note that the distributions are fairly stable despite the increase of data and, in particular, the exponents of the power-law tails are evidently invariant. They are respectively –2.2 for $k$ (the number of trading partners), –2.2 for $l$ (employee number) and –2.0 for $s$ (annual sales in million yen). The exponent of sales distribution is consistent with previous studies [1–3]. Consequently, arithmetic mean and standard deviation do not indicate the representative value and the width of the distribution (Table S1). We alternatively measure them by the median and the IQR (interquartile range) in the table. Note, however, that these values are only representative of middle-range values, but not the tails, where considerably regular characteristics appear.

In Fig. S3, we also plot the distribution of firm growth rates $g_x(t) = x(t)/x(t–1)$ of a single variable $x$ in one year, where $x$ is one of the size variables $k$, $l$ and $s$ and $t$ is the year. The zigzagged forms at the center of $k$ and $l$ distributions in Figs. S3a and S3b are due to the fact that the number of trading partners or employees are integer, and a very large fraction of firms have only a few trading partners or employees (Fig. S2a,b). Again, consistent to the previous studies [4,5], the distributions of log-transformed growth rates $\log[g_x(t)]$ are approximately Laplace or double exponential. This means that the tails of both sides of non-transformed growth rates are approximated with power-laws and one can obtain an extreme value larger or smaller than a unity by several orders of magnitude.

To assure that the scaling relationships that were found in the previous study [6] are also present in our data, we follow the methodology described there to replicate their results. The data in the previous study were independently gathered from the data provider in our study, Teikoku Databank, Ltd. However, we expect that similar results would emerge, as data are collected for the same system (i.e. the Japanese firms) in both datasets.

Firstly, we confirm the following scaling relationships, which is defined in terms of conditional distributions [6]:

$$\mathrm{P}(l|k) = \tilde{P}_{l|k}(l/k^{\gamma_1})/k^{\gamma_1}, \tag{S2.1}$$

$$\mathrm{P}(s|k) = \tilde{P}_{s|k}(s/k^{\gamma_2})/k^{\gamma_2}, \tag{S2.2}$$

$$\mathrm{P}(s|l) = \tilde{P}_{s|l}(s/l^{\gamma_3})/l^{\gamma_3}, \tag{S2.3}$$

where $\mathrm{P}(x|y)$ is the probability density function of the variable $x$ conditional on a specific $y$-value, $\gamma_1$, $\gamma_2$ and $\gamma_3$ are the scaling exponents, and $\tilde{P}_{x|y}$ is a scaling function for variable $x$ conditional on the $y$-value, which represents the distribution of fluctuation ratio around the scaling line, $x \propto y^{\gamma}$. These relations are equivalent to the more intuitive regression-type formulae as shown in Supplementary Text 4:

$$\log l = \gamma_1 \log k + \varepsilon_{l|k}, \tag{S2.4}$$

$$\log s = \gamma_2 \log k + \varepsilon_{s|k}, \tag{S2.5}$$

$$\log s = \gamma_3 \log l + \varepsilon_{s|l}, \tag{S2.6}$$

where the error terms, $\varepsilon_{l|k}$, $\varepsilon_{s|k}$ and $\varepsilon_{s|l}$, can be regarded as stochastic variables (including the intercept term) that correspond to $\tilde{P}_{l|k}$, $\tilde{P}_{s|k}$ and $\tilde{P}_{s|l}$. These formulae are naturally interpreted as projections of a single 3-dimensional scaling line, where the firms are densely distributed, to the 2-dimensional planes (Fig. 3a).

To test the validity of these relationships (Eqs. (S2.1–6)) in our data, we examine both the conditional quantiles (Fig. S4a–c) and the distributions of the error terms (Fig. S4d–f), where the conditional quantile is defined as follows: for any given number $q$ in the range of (0, 1), the $q$-quantile of $x$ conditional on $y$, denoted as $\langle x|y\rangle_q$, is defined by the value that fulfills the following equation,

$$\int_0^{\langle x|y\rangle_q} \mathrm{P}(x|y)\,\mathrm{d}x = q. \tag{S2.7}$$

As shown in Fig. S4a–c, the plots of $\log\langle x|y\rangle_q$ vs $\log y$ show linear relations for a wide range of $y$, meaning that the power law relation, $\langle x|y\rangle_q \propto y^{\gamma}$, shortly denoted by $x \propto y^{\gamma}$, holds for all combinations of $k$, $l$ and $s$. We estimate the values of exponents as $\gamma_1 \sim 1.0$, $\gamma_2 \sim 1.2$, and $\gamma_3 \sim 1.2$ (Supplementary Text 4). In Fig. S4d–f, we plot the scaling functions, $\tilde{P}_{x|y}$, for 8 intervals of a logarithmically equal range of $y$, and confirm that all the curves collapse into a single scaling function for all three cases, demonstrating the validity of the scaling relations of Eqs. (S2.1–3).

In this note, we derive the asymptotic exponents of power-law distributions and scaling relationships from other

ones to check the consistency of our results. First, given Eqs. (S2.1–3), we derive the asymptotic power-law exponent of the marginal distribution $\mathrm{P}(x)$ of the 'explained' variable *x*. Second, assuming Eqs. (3) and (S2.1), we calculate the asymptotic power-law exponent of marginal distribution of *s*. Third, we show that the bivariate scaling exponents $\gamma_2$ and $\gamma_3$ (i.e. those of the sales *s* against the number of trading partners *k* and against employee number *l* respectively) can be determined from $\alpha$, $\beta$ and $\gamma_1$.

Since Eqs. (S2.1–3) have the general form

$$\mathrm{P}(x|y) = \tilde{P}_{x|y}(x/y^{\gamma})/y^{\gamma}\,, \tag{S3.1}$$

we can derive the power-law exponent of the marginal distribution $P_x(x)$ of a variable *x* from the following three: the positive scaling exponent $\gamma$, $\tilde{P}_{x|y}$ (the universal distribution function of *x* conditional on *y*) and the marginal distribution $P_y(y)$. Assuming that $\tilde{P}_{x|y}$ and $P_y$ has a power-law upper tail of exponent $\delta_{x|y}$ and $\delta_y$, we approximate the functions as

$$\tilde{P}_{x|y}(\tilde{x}) = \begin{cases} c_{x|y}\tilde{x}^{-\delta_{x|y}} & (\tilde{x} \geq 1) \\ d_{x|y}(\tilde{x}) & (0 \leq \tilde{x} < 1) \end{cases} \tag{S3.2}$$

and

$$P_y(y) = \begin{cases} c_y y^{-\delta_y} & (y \geq 1) \\ d_y(y) & (0 \leq y < 1) \end{cases}, \tag{S3.3}$$

where $c_{x|y}$ and $c_y$ are positive constants, $\delta_{x|y}$ and $\delta_y$ are the power-law exponents larger than 1 and $d_{x|y}$ and $d_y$ are the distribution functions at the smaller side. This approximation is motivated by the actual distributions of size variables (Figs. 2d–f and S2). We set the threshold beyond which the distribution follow the power law to 1, since, otherwise, the same results are easily derived for the asymptotic value of exponents with linear transformations.

Applying Bayes' theorem and assuming $x > 1$ (as we are interested in the 'tails' or asymptotic behaviors at $x \to \infty$), we derive $P_x(x)$, the marginal distribution of *x*, from $\mathrm{P}(x, y)$, the joint distribution of *x* and *y*:

$$\begin{aligned}
P_x(x) &= \int_0^{\infty} \mathrm{P}(x,y)\mathrm{d}y = \int_0^{\infty} \mathrm{P}(x|y)\mathrm{P}(y)\mathrm{d}y = \int_0^{\infty} \frac{1}{y^{\gamma}} \tilde{P}_{x|y}\left(\frac{x}{y^{\gamma}}\right) P_y(y)\mathrm{d}y \\
&= \int_0^{1} \frac{1}{y^{\gamma}} c_{x|y} \left(\frac{x}{y^{\gamma}}\right)^{-\delta_{x|y}} d_y(y)\mathrm{d}y + \int_1^{x^{1/\gamma}} \frac{1}{y^{\gamma}} c_{x|y} \left(\frac{x}{y^{\gamma}}\right)^{-\delta_{x|y}} c_y y^{-\delta_y}\mathrm{d}y + \int_{x^{1/\gamma}}^{\infty} \frac{1}{y^{\gamma}} d_{x|y}\left(\frac{x}{y^{\gamma}}\right) c_y y^{-\delta_y}\mathrm{d}y \\
&= c_{x|y} x^{-\delta_{x|y}} \int_0^1 y^{\gamma(\delta_{x|y}-1)} d_y(y)\mathrm{d}y + c_{x|y} c_y x^{-\delta_{x|y}} \int_1^{x^{1/\gamma}} y^{\gamma(\delta_{x|y}-1)-\delta_y}\mathrm{d}y \\
&\qquad + c_y x^{-(\delta_y-1)/\gamma-1} \int_1^{\infty} \tilde{y}^{-\gamma-\delta_y} d_{x|y}\left(\frac{1}{\tilde{y}^{\gamma}}\right)\mathrm{d}\tilde{y} \\
&= (I_1 - C)x^{-\delta_{x|y}} + (I_2 + C)x^{-1-(\delta_y-1)/\gamma},
\end{aligned}$$

where $I_1$, $I_2$ and $C$ are constants defined as

$$I_1 = c_{x|y} \int_0^1 y^{\gamma(\delta_{x|y}-1)} d_y(y)\mathrm{d}y\,,$$

$$I_2 = c_y \int_1^{\infty} \tilde{y}^{-\gamma-\delta_y} d_{x|y}\left(\frac{1}{\tilde{y}^{\gamma}}\right) \mathrm{d}\tilde{y},$$

$$C = c_{x|y} c_y / \left(\gamma(\delta_{x|y} - 1) - \delta_y + 1\right),$$

and the substitution $\tilde{y} = y/x^{1/\gamma}$ is applied in the last integral term. Therefore, the asymptotic behavior of $P_x(x)$ at positive infinity is determined by which of $-\delta_{x|y}$ and $-1 - (\delta_y - 1)/\gamma$ is the larger: when $x \to \infty$, the behavior of $P_x$ is approximated with

$$P_x(x) \propto x^{-\delta_x}, \tag{S3.4}$$

where

$$-\delta_x = \max\left[-\delta_{x|y}, \quad -1 - \frac{\delta_y - 1}{\gamma}\right]. \tag{S3.5}$$

Note that change of $\delta_{x|y}$ does not have any effect on the power-law exponent as far as $\delta_y$ is sufficiently large, which is consistent to the intuitive explanation (Fig. 1) in the main text.

Although somewhat complicated, a similar strategy works for the case of multi-variate scaling. Let us continue with the above notations except that $x$, $y$ and $\gamma$ are respectively replaced with $l$, $k$ and $\gamma_1$, and assume Eq. (3) as well as the following:

$$\tilde{P}_{s|k,l}(\tilde{s}) = \begin{cases} c_{s|k,l}\tilde{s}^{-\delta_{s|k,l}} & (\tilde{s} \geq 1) \\ d_{s|k,l}(\tilde{s}) & (0 \leq \tilde{s} < 1) \end{cases}, \tag{S3.6}$$

where $c_{s|l,k}$ is a positive constant, $\delta_{s|k,l}$ the power-law exponent larger than 1 and $d_{s|k,l}$ the distribution function at the smaller side. Again, the threshold of the functional change of $\tilde{P}_{s|k,l}$ is set to a unity without loss of generality. The marginal distribution of $s$, $P_s(s)$, for $s > 1$ is

$$P_s(s) = \int_0^{\infty}\int_0^{\infty} \mathrm{P}(k,l,s)\mathrm{d}l\,\mathrm{d}k = \int_0^{\infty}\int_0^{\infty} \mathrm{P}(s|k,l)\mathrm{P}(k,l)\mathrm{d}l\,\mathrm{d}k = \int_0^{\infty}\int_0^{\infty} \mathrm{P}(s|k,l)\mathrm{P}(l|k)\mathrm{P}(k)\mathrm{d}l\,\mathrm{d}k.$$

Then, this is calculated as the sum of following ten integral terms:

$$\int_0^1\int_0^{k^{\gamma_1}} \mathrm{P}(s|k,l)\mathrm{P}(l|k)\mathrm{P}(k)\mathrm{d}l\,\mathrm{d}k = \int_0^1\int_0^{k^{\gamma_1}} \frac{1}{k^{\alpha}l^{\beta}} c_{s|k,l}\left(\frac{s}{k^{\alpha}l^{\beta}}\right)^{-\delta_{s|k,l}} \frac{1}{k^{\gamma_1}} d_{l|k}\left(\frac{l}{k^{\gamma_1}}\right) d_k(k)\mathrm{d}l\,\mathrm{d}k$$

$$= c_{s|k,l}s^{-\delta_{s|k,l}} \int_0^1 k^{-\gamma_1+\alpha(\delta_{s|k,l}-1)} d_k(k) \int_0^{k^{\gamma_1}} l^{\beta(\delta_{s|k,l}-1)} d_{l|k}\left(\frac{l}{k^{\gamma_1}}\right)\mathrm{d}l\,\mathrm{d}k$$

$$= \left[c_{s|k,l}\int_0^1 k^{(\alpha+\beta\gamma_1)(\delta_{s|k,l}-1)} d_k(k) \int_0^1 \tilde{l}^{\beta(\delta_{s|k,l}-1)} d_{l|k}(\tilde{l})\mathrm{d}\tilde{l}\,\mathrm{d}k\right] s^{-\delta_{s|k,l}},$$

where the substitution $\tilde{l} = l/k^{\gamma_1}$ is applied;

$$\int_0^1\int_{k^{\gamma_1}}^{(s/k^{\alpha})^{1/\beta}} \mathrm{P}(s|k,l)\mathrm{P}(l|k)\mathrm{P}(k)\mathrm{d}l\,\mathrm{d}k$$

$$= \int_0^1\int_{k^{\gamma_1}}^{(s/k^{\alpha})^{1/\beta}} \frac{1}{k^{\alpha}l^{\beta}} c_{s|k,l}\left(\frac{s}{k^{\alpha}l^{\beta}}\right)^{-\delta_{s|k,l}} \frac{1}{k^{\gamma_1}} c_{l|k}\left(\frac{l}{k^{\gamma_1}}\right)^{-\delta_{l|k}} d_k(k)\mathrm{d}l\,\mathrm{d}k$$

$$= c_{l|k}c_{s|k,l}s^{-\delta_{s|k,l}} \int_0^1 k^{\alpha(\delta_{s|k,l}-1)+\gamma_1(\delta_{l|k}-1)} d_k(k) \int_{k^{\gamma_1}}^{(s/k^{\alpha})^{1/\beta}} l^{\beta(\delta_{s|k,l}-1)-\delta_{l|k}}\mathrm{d}l\,\mathrm{d}k$$

$$= \frac{c_{l|k} c_{s|k,l}}{E_1} \left( \left[ \int_0^1 k^{(\alpha/\beta+\gamma_1)(\delta_{l|k}-1)} d_k(k) \mathrm{d}k \right] s^{-1-(\delta_{l|k}-1)/\beta} - \left[ \int_0^1 k^{(\alpha+\beta\gamma_1)(\delta_{s|k,l}-1)} d_k(k) \mathrm{d}k \right] s^{-\delta_{s|k,l}} \right),$$

where $E_1 = \beta(\delta_{s|k,l} - 1) - \delta_{l|k} + 1$;

$$\int_0^1 \int_{\left(\frac{s^\alpha}{k}\right)^{\frac{1}{\beta}}}^\infty \mathrm{P}(s|k,l)\mathrm{P}(l|k)\mathrm{P}(k) \mathrm{d}l \, \mathrm{d}k = \int_0^1 \int_{\left(\frac{s^\alpha}{k}\right)^{\frac{1}{\beta}}}^\infty \frac{1}{k^\alpha l^\beta} d_{s|k,l} \left( \frac{s}{k^\alpha l^\beta} \right) \frac{1}{k^{\gamma_1}} c_{l|k} \left( \frac{l}{k^{\gamma_1}} \right)^{-\delta_{l|k}} d_k(k) \mathrm{d}l \, \mathrm{d}k$$

$$= c_{l|k} \int_0^1 k^{\gamma_1(\delta_{l|k}-1)-\alpha} d_k(k) \int_{(s/k^\alpha)^{1/\beta}}^\infty d_{s|k,l} \left( \frac{s}{k^\alpha l^\beta} \right) l^{-\delta_{l|k}-\beta} \mathrm{d}l \, \mathrm{d}k$$

$$= \left[ c_{l|k} \int_0^1 k^{(\alpha/\beta+\gamma_1)(\delta_{l|k}-1)} d_k(k) \mathrm{d}k \int_1^\infty d_{s|k,l} \left( \frac{1}{\tilde{l}^\beta} \right) \tilde{l}^{-\delta_{l|k}-\beta} \mathrm{d}\tilde{l} \right] s^{-1-(\delta_{l|k}-1)/\beta},$$

where the substitution $\tilde{l} = \left( k^{\alpha/\beta} / s^{1/\beta} \right) \cdot l$ is applied;

$$\int_1^{s^{1/(\alpha+\beta\gamma_1)}} \int_0^{k^{\gamma_1}} \mathrm{P}(s|k,l)\mathrm{P}(l|k)\mathrm{P}(k) \mathrm{d}l \, \mathrm{d}k$$

$$= \int_1^{s^{1/(\alpha+\beta\gamma_1)}} \int_0^{k^{\gamma_1}} \frac{1}{k^\alpha l^\beta} c_{s|k,l} \left( \frac{s}{k^\alpha l^\beta} \right)^{-\delta_{s|k,l}} \frac{1}{k^{\gamma_1}} d_{l|k} \left( \frac{l}{k^{\gamma_1}} \right) c_k k^{-\delta_k} \mathrm{d}l \, \mathrm{d}k$$

$$= c_k c_{s|k,l} s^{-\delta_{s|k,l}} \int_1^{s^{1/(\alpha+\beta\gamma_1)}} k^{\alpha(\delta_{s|k,l}-1)-\gamma_1-\delta_k} \int_0^{k^{\gamma_1}} l^{\beta(\delta_{s|k,l}-1)} d_{l|k} \left( \frac{l}{k^{\gamma_1}} \right) \mathrm{d}l \, \mathrm{d}k$$

$$= \frac{c_k c_{s|k,l}}{E_2} \left[ \int_0^1 \tilde{l}^{\beta(\delta_{s|k,l}-1)} d_{l|k}(\tilde{l}) \mathrm{d}\tilde{l} \right] \left( s^{-1-(\delta_k-1)/(\alpha+\beta\gamma_1)} - s^{-\delta_{s|k,l}} \right),$$

where the substitution $\tilde{l} = l/k^{\gamma_1}$ is applied and $E_2 = (\alpha + \beta\gamma_1)(\delta_{s|k,l} - 1) - \delta_k + 1$;

$$\int_1^{s^{1/(\alpha+\beta\gamma_1)}} \int_{k^{\gamma_1}}^{(s/k^\alpha)^{1/\beta}} \mathrm{P}(s|k,l)\mathrm{P}(l|k)\mathrm{P}(k) \mathrm{d}l \, \mathrm{d}k$$

$$= \int_1^{s^{1/(\alpha+\beta\gamma_1)}} \int_{k^{\gamma_1}}^{(s/k^\alpha)^{1/\beta}} \frac{1}{k^\alpha l^\beta} c_{s|k,l} \left( \frac{s}{k^\alpha l^\beta} \right)^{-\delta_{s|k,l}} \frac{1}{k^{\gamma_1}} c_{l|k} \left( \frac{l}{k^{\gamma_1}} \right)^{-\delta_{l|k}} c_k k^{-\delta_k} \mathrm{d}l \, \mathrm{d}k$$

$$= c_k c_{l|k} c_{s|k,l} s^{-\delta_{s|k,l}} \int_1^{s^{1/(\alpha+\beta\gamma_1)}} k^{\alpha(\delta_{s|k,l}-1)+\gamma_1(\delta_{l|k}-1)-\delta_k} \int_{k^{\gamma_1}}^{(s/k^\alpha)^{1/\beta}} l^{\beta(\delta_{s|k,l}-1)-\delta_{l|k}} \mathrm{d}l \, \mathrm{d}k$$

$$= \frac{c_k c_{l|k} c_{s|k,l}}{E_1} \left( \left( \frac{1}{E_3} - \frac{1}{E_2} \right) s^{-1-(\delta_k-1)/(\alpha+\beta\gamma_1)} - \frac{1}{E_3} s^{-1-(\delta_{l|k}-1)/\beta} + \frac{1}{E_2} s^{-\delta_{s|k,l}} \right),$$

where $E_3 = (\alpha/\beta + \gamma_1)(\delta_{l|k} - 1) - \delta_k + 1$;

$$\int_1^{s^{1/(\alpha+\beta\gamma_1)}} \int_{(s/k^\alpha)^{1/\beta}}^\infty \mathrm{P}(s|k,l)\mathrm{P}(l|k)\mathrm{P}(k) \mathrm{d}l \, \mathrm{d}k$$

$$= \int_1^{s^{1/(\alpha+\beta\gamma_1)}} \int_{(s/k^\alpha)^{1/\beta}}^\infty \frac{1}{k^\alpha l^\beta} d_{s|k,l} \left( \frac{s}{k^\alpha l^\beta} \right) \frac{1}{k^{\gamma_1}} c_{l|k} \left( \frac{l}{k^{\gamma_1}} \right)^{-\delta_{l|k}} c_k k^{-\delta_k} \mathrm{d}l \, \mathrm{d}k$$

$$= c_k c_{l|k} \int_1^{s^{1/(\alpha+\beta\gamma_1)}} k^{-\alpha+\gamma_1(\delta_{l|k}-1)-\delta_k} \int_{(s/k^\alpha)^{1/\beta}}^\infty \frac{1}{l^\beta} d_{s|k,l} \left( \frac{s}{k^\alpha l^\beta} \right) l^{-\delta_{l|k}} \mathrm{d}l \, \mathrm{d}k$$

$$= \left[ \frac{c_k c_{l|k}}{E_3} \int_1^\infty d_{s|k,l} \left( \frac{1}{\tilde{l}^\beta} \right) \tilde{l}^{-\delta_{l|k}-\beta} \mathrm{d}\tilde{l} \right] \left( s^{-1-(\delta_k-1)/(\alpha+\beta\gamma_1)} - s^{-1-(\delta_{l|k}-1)/\beta} \right),$$

where the substitution $\tilde{l} = \left(k^{\alpha/\beta}/s^{1/\beta}\right) \cdot l$ is applied;

$$\begin{aligned}
&\int_0^{s^{\gamma_1/(\alpha+\beta\gamma_1)}} \int_{s^{1/(\alpha+\beta\gamma_1)}}^{(s/l^\beta)^{1/\alpha}} \mathrm{P}(s|k,l)\mathrm{P}(l|k)\mathrm{P}(k)\mathrm{d}k\,\mathrm{d}l \\
&= \int_0^{s^{\gamma_1/(\alpha+\beta\gamma_1)}} \int_{s^{1/(\alpha+\beta\gamma_1)}}^{(s/l^\beta)^{1/\alpha}} \frac{1}{k^\alpha l^\beta} c_{s|k,l} \left(\frac{s}{k^\alpha l^\beta}\right)^{-\delta_{s|k,l}} \frac{1}{k^{\gamma_1}} d_{l|k} \left(\frac{l}{k^{\gamma_1}}\right) c_k k^{-\delta_k} \mathrm{d}k\,\mathrm{d}l \\
&= \left(c_k c_{s|k,l} I_1^3\right) s^{-1-(\delta_k-1)/(\alpha+\beta\gamma_1)},
\end{aligned}$$

where

$$I_1^3 = \int_0^1 \tilde{l}^{-1+(\delta_{s|k,l}-1)(\alpha+\beta\gamma_1)/\gamma_1-(\delta_k-1)/\gamma_1} \int_{\tilde{l}^{-1/\gamma_1}}^{\tilde{l}^{-(\alpha+\beta\gamma_1)/\alpha\gamma_1}} \tilde{k}^{\alpha(\delta_{s|k,l}-1)-\gamma_1-\delta_k} d_{l|k} \left(\frac{1}{\tilde{k}^{\gamma_1}}\right) \mathrm{d}\tilde{k}\,\mathrm{d}\tilde{l}$$

and the substitutions $\tilde{k} = l^{-1/\gamma_1} \cdot k$ and $\tilde{l} = s^{-\gamma_1/(\alpha+\beta\gamma_1)} \cdot l$ are applied;

$$\begin{aligned}
&\int_0^{s^{\gamma_1/(\alpha+\beta\gamma_1)}} \int_{(s/l^\beta)^{1/\alpha}}^{\infty} \mathrm{P}(s|k,l)\mathrm{P}(l|k)\mathrm{P}(k)\mathrm{d}k\,\mathrm{d}l \\
&= \int_0^{s^{\gamma_1/(\alpha+\beta\gamma_1)}} \int_{(s/l^\beta)^{1/\alpha}}^{\infty} \frac{1}{k^\alpha l^\beta} d_{s|k,l} \left(\frac{s}{k^\alpha l^\beta}\right) \frac{1}{k^{\gamma_1}} d_{l|k} \left(\frac{l}{k^{\gamma_1}}\right) c_k k^{-\delta_k} \mathrm{d}k\,\mathrm{d}l \\
&= \left(c_k I_2^3\right) s^{-1-(\delta_k-1)/(\alpha+\beta\gamma_1)},
\end{aligned}$$

where

$$I_2^3 = \int_0^1 \tilde{l}^{(\gamma_1+\delta_k-1)\beta/\alpha} \int_1^\infty \frac{1}{\tilde{k}^\alpha} d_{s|k,l} \left(\frac{1}{\tilde{k}^\alpha}\right) \frac{1}{\tilde{k}^{\gamma_1}} d_{s|k,l} \left(\frac{\tilde{l}^{(\alpha+\beta\gamma_1)/\alpha}}{\tilde{k}^{\gamma_1}}\right) \tilde{k}^{-\delta_k} \mathrm{d}\tilde{k}\,\mathrm{d}\tilde{l}$$

and the substitutions $\tilde{k} = \left(l^\beta/s\right)^{1/\alpha} \cdot k$ and $\tilde{l} = s^{-\gamma_1/(\alpha+\beta\gamma_1)} \cdot l$ are applied;

$$\begin{aligned}
&\int_{s^{\gamma_1/(\alpha+\beta\gamma_1)}}^{\infty} \int_{l^{1/\gamma_1}}^{\infty} \mathrm{P}(s|k,l)\mathrm{P}(l|k)\mathrm{P}(k)\mathrm{d}k\,\mathrm{d}l \\
&= \int_{s^{\gamma_1/(\alpha+\beta\gamma_1)}}^{\infty} \int_{l^{1/\gamma_1}}^{\infty} \frac{1}{k^\alpha l^\beta} d_{s|k,l} \left(\frac{s}{k^\alpha l^\beta}\right) \frac{1}{k^{\gamma_1}} d_{l|k} \left(\frac{l}{k^{\gamma_1}}\right) c_k k^{-\delta_k} \mathrm{d}k\,\mathrm{d}l \\
&= \left(c_k I_3^3\right) s^{-1-(\delta_k-1)/(\alpha+\beta\gamma_1)},
\end{aligned}$$

where

$$I_3^3 = \int_1^\infty \tilde{l}^{-1-(\alpha+\beta\gamma_1+\delta_k-1)/\gamma_1} \int_1^\infty \frac{1}{\tilde{k}^\alpha} d_{s|k,l} \left(\frac{1}{\tilde{k}^\alpha \tilde{l}^{(\alpha+\beta\gamma_1)/\gamma_1}}\right) \frac{1}{\tilde{k}^{\gamma_1}} d_{s|k,l} \left(\frac{1}{\tilde{k}^{\gamma_1}}\right) \tilde{k}^{-\delta_k} \mathrm{d}\tilde{k}\,\mathrm{d}\tilde{l}$$

and the substitutions $\tilde{k} = l^{-1/\gamma_1} \cdot k$ and $\tilde{l} = s^{-\gamma_1/(\alpha+\beta\gamma_1)} \cdot l$ are applied;

$$\begin{aligned}
&\int_{s^{\gamma_1/(\alpha+\beta\gamma_1)}}^{\infty} \int_{s^{1/(\alpha+\beta\gamma_1)}}^{l^{1/\gamma_1}} \mathrm{P}(s|k,l)\mathrm{P}(l|k)\mathrm{P}(k)\mathrm{d}k\,\mathrm{d}l \\
&= \int_{s^{\gamma_1/(\alpha+\beta\gamma_1)}}^{\infty} \int_{s^{1/(\alpha+\beta\gamma_1)}}^{l^{1/\gamma_1}} \frac{1}{k^\alpha l^\beta} d_{s|k,l} \left(\frac{s}{k^\alpha l^\beta}\right) \frac{1}{k^{\gamma_1}} c_{l|k} \left(\frac{l}{k^{\gamma_1}}\right)^{-\delta_{l|k}} c_k k^{-\delta_k} \mathrm{d}k\,\mathrm{d}l \\
&= \left(c_k c_{l|k} I_4^3\right) s^{-1-(\delta_k-1)/(\alpha+\beta\gamma_1)},
\end{aligned}$$

where

$$I_4^3 = \int_1^\infty \tilde{l}^{-1-(\alpha+\beta\gamma_1+\delta_k-1)/\gamma_1} \int_{\tilde{l}^{-1/\gamma_1}}^{1} \frac{1}{\tilde{k}^\alpha} d_{s|k,l} \left(\frac{1}{\tilde{k}^\alpha \tilde{l}^{(\alpha+\beta\gamma_1)/\gamma_1}}\right) \tilde{k}^{\gamma_1(\delta_{l|k}-1)-\delta_k} \mathrm{d}\tilde{k}\,\mathrm{d}\tilde{l}$$

and the substitutions $\tilde{k} = l^{-1/\gamma_1} \cdot k$ and $\tilde{l} = s^{-\gamma_1/(\alpha+\beta\gamma_1)} \cdot l$ are applied. We note that the final sum of these ten terms has the form

$$P_s(s) = A_1 \cdot s^{-\delta_{s|k,l}} + A_2 \cdot s^{-1-\frac{\delta_{l|k}-1}{\beta}} + A_3 \cdot s^{-1-\frac{\delta_k-1}{\alpha+\beta\gamma_1}},$$

where $A_1$, $A_2$ and $A_3$ are independent of $s$. Therefore, the asymptotic behavior of $P_s$ at $s \to \infty$ is that

$$P_s(s) \propto s^{-\delta_s}, \tag{S3.7}$$

where $-\delta_s$ is the largest of the three exponents:

$$-\delta_s = \max\left[-\delta_{s|k,l}, \quad -1 - \frac{\delta_{l|k} - 1}{\beta}, \quad -1 - \frac{\delta_k - 1}{\alpha + \beta\gamma_1}\right]. \tag{S3.8}$$

Lastly, we evaluate the values of the exponents $\gamma_2$ and $\gamma_3$ from $\alpha$, $\beta$ and $\gamma_1$. Again, assume Eqs. (2) and (S2.1). Then, the joint distribution of $k$, $l$ and $s$ is given by

$$\mathrm{P}(k,l,s) = \mathrm{P}(s|k,l)\mathrm{P}(l|k)\mathrm{P}(k) = \frac{1}{k^\alpha l^\beta}\tilde{P}_{s|k,l}\left(\frac{s}{k^\alpha l^\beta}\right)\frac{1}{k^{\gamma_1}}\tilde{P}_{l|k}\left(\frac{l}{k^{\gamma_1}}\right)P_k(k).$$

We can obtain the joint distribution of $k$ and $s$ by integrating this probability by $l$.

$$\mathrm{P}(k,s) = \int_{-\infty}^{\infty}\mathrm{P}(k,l,s)\mathrm{d}l = \int_0^{\infty}\frac{1}{k^\alpha l^\beta}\tilde{P}_{s|k,l}\left(\frac{s}{k^\alpha l^\beta}\right)\frac{1}{k^{\gamma_1}}\tilde{P}_{l|k}\left(\frac{l}{k^{\gamma_1}}\right)P_k(k)\mathrm{d}l.$$

Now,

$$\mathrm{P}(k = k_0, s) = \int_0^{\infty}\frac{1}{{k_0}^\alpha l^\beta}\tilde{P}_{s|k,l}\left(\frac{s}{{k_0}^\alpha l^\beta}\right)\frac{1}{{k_0}^{\gamma_1}}\tilde{P}_{l|k}\left(\frac{l}{{k_0}^{\gamma_1}}\right)P_k(k_0)\mathrm{d}l$$

and

$$\begin{aligned}\mathrm{P}(k = k_1, s) &= \int_0^{\infty}\frac{1}{{k_1}^\alpha l^\beta}\tilde{P}_{s|k,l}\left(\frac{s}{{k_1}^\alpha l^\beta}\right)\frac{1}{{k_1}^{\gamma_1}}\tilde{P}_{l|k}\left(\frac{l}{{k_1}^{\gamma_1}}\right)P_k(k_1)\mathrm{d}l \\ &= \left(\frac{k_0}{k_1}\right)^{\alpha+\beta\gamma_1}\cdot\frac{P_k(k_1)}{P_k(k_0)}\int_0^{\infty}\frac{1}{{k_0}^\alpha \tilde{l}^\beta}\tilde{P}_{s|k,l}\left(\frac{s}{{k_0}^\alpha \tilde{l}^\beta}\cdot\left(\frac{k_0}{k_1}\right)^{\alpha+\beta\gamma_1}\right)\frac{1}{{k_0}^{\gamma_1}}\tilde{P}_{l|k}\left(\frac{\tilde{l}}{{k_0}^{\gamma_1}}\right)P_k(k_0)\mathrm{d}\tilde{l} \\ &= \left(\frac{k_0}{k_1}\right)^{\alpha+\beta\gamma_1}\cdot\frac{P_k(k_1)}{P_k(k_0)}\cdot\mathrm{P}\left(k = k_0, \quad s = \left(\frac{k_0}{k_1}\right)^{\alpha+\beta\gamma_1}s\right),\end{aligned}$$

where the substitution $\tilde{l} = (k_0/k_1)^{\gamma_1} \cdot l$ is used. Here,

$$\begin{aligned}\mathrm{P}(s|k = k_1) = \frac{\mathrm{P}(s,k_1)}{\mathrm{P}(k_1)} &= \frac{1}{{k_1}^{\alpha+\beta\gamma_1}}\cdot\frac{{k_0}^{\alpha+\beta\gamma_1}}{P_k(k_0)}\cdot\mathrm{P}\left(k = k_0, \quad s = {k_0}^{\alpha+\beta\gamma_1}\cdot\frac{s}{{k_1}^{\alpha+\beta\gamma_1}}\right) \\ &= \frac{1}{{k_1}^{\alpha+\beta\gamma_1}}\tilde{P}_{s|k}\left(\frac{s}{{k_1}^{\alpha+\beta\gamma_1}}\right),\end{aligned}$$

where

$$\tilde{P}_{s|k}(\tilde{s}) = \frac{{k_0}^{\alpha+\beta\gamma_1}}{P_k(k_0)}\cdot\mathrm{P}\left(k = k_0, \quad s = {k_0}^{\alpha+\beta\gamma_1}\cdot\tilde{s}\right).$$

Comparing the result above with Eq. (S2.2), we have

$$\gamma_2 = \alpha + \beta\gamma_1\,. \tag{S3.9}$$

Similarly, the joint distribution of $l$ and $s$ is determined with the equation

$$\mathrm{P}(l,s)=\int_{-\infty}^{\infty}\mathrm{P}(k,l,s)\mathrm{d}k=\int_{0}^{\infty}\frac{1}{k^{\alpha}l^{\beta}}\tilde{P}_{s|k,l}\left(\frac{s}{k^{\alpha}l^{\beta}}\right)\frac{1}{k^{\gamma_1}}\tilde{P}_{l|k}\left(\frac{l}{k^{\gamma_1}}\right)P_k(k)\mathrm{d}k,$$

and, as a result,

$$\mathrm{P}(l=l_0,s)=\int_{0}^{\infty}\frac{1}{k^{\alpha}{l_0}^{\beta}}\tilde{P}_{s|k,l}\left(\frac{s}{k^{\alpha}{l_0}^{\beta}}\right)\frac{1}{k^{\gamma_1}}\tilde{P}_{l|k}\left(\frac{l}{k^{\gamma_1}}\right)P_k(k)\mathrm{d}k$$

and

$$\begin{aligned}\mathrm{P}(l=l_1,s)&=\int_{0}^{\infty}\frac{1}{k^{\alpha}{l_1}^{\beta}}\tilde{P}_{s|k,l}\left(\frac{s}{k^{\alpha}{l_1}^{\beta}}\right)\frac{1}{k^{\gamma_1}}\tilde{P}_{l|k}\left(\frac{l}{k^{\gamma_1}}\right)P_k(k)\mathrm{d}k\\&=\left(\frac{l_0}{l_1}\right)^{(\gamma_1-1+\alpha+\beta\gamma_1)/\gamma_1}\cdot\int_{0}^{\infty}\frac{1}{\tilde{k}^{\alpha}{l_0}^{\beta}}\tilde{P}_{s|k,l}\left(\frac{s}{\tilde{k}^{\alpha}{l_0}^{\beta}}\cdot\left(\frac{l_0}{l_1}\right)^{(\alpha+\beta\gamma_1)/\gamma_1}\right)\frac{1}{\tilde{k}^{\gamma_1}}\tilde{P}_{l|k}\left(\frac{l_0}{\tilde{k}^{\gamma_1}}\right)P_k\left(\tilde{k}\cdot\left(\frac{l_1}{l_0}\right)^{1/\gamma_1}\right)\mathrm{d}\tilde{k},\end{aligned}$$

where the substitution $\tilde{k}=(l_0/l_1)^{1/\gamma_1}\cdot k$ is used. Then, if we assume the power law distribution of $k$ comparable to Eq. (S3.3), namely

$$P_k(k)=\begin{cases}c_k k^{-\delta_k} & (y\geq\theta_k)\\ d_k(k) & (0\leq y<\theta_k)\end{cases},$$

where $\theta_k$ is a positive constant of the threshold,

$$\begin{aligned}&\mathrm{P}(l=l_1,s)\\&=\left(\frac{l_0}{l_1}\right)^{(\gamma_1-1+\alpha+\beta\gamma_1)/\gamma_1}\left[\left(\frac{l_0}{l_1}\right)^{\delta_k/\gamma_1}\mathrm{P}\left(l=l_0,\left(\frac{l_0}{l_1}\right)^{(\alpha+\beta\gamma_1)/\gamma_1}s\right)\right.\\&\qquad\left.-\int_{0}^{\theta_k}\frac{1}{\tilde{k}^{\alpha}{l_0}^{\beta}}\tilde{P}_{s|k,l}\left(\frac{s}{\tilde{k}^{\alpha}{l_0}^{\beta}}\cdot\left(\frac{l_0}{l_1}\right)^{(\alpha+\beta\gamma_1)/\gamma_1}\right)\frac{1}{\tilde{k}^{\gamma_1}}\tilde{P}_{l|k}\left(\frac{l_0}{\tilde{k}^{\gamma_1}}\right)P_k(\tilde{k})\mathrm{d}\tilde{k}\right]\\&\qquad+\int_{0}^{\theta_k(l_1/l_0)^{1/\gamma_1}}\frac{1}{k^{\alpha}{l_1}^{\beta}}\tilde{P}_{s|k,l}\left(\frac{s}{k^{\alpha}{l_1}^{\beta}}\right)\frac{1}{k^{\gamma_1}}\tilde{P}_{l|k}\left(\frac{l}{k^{\gamma_1}}\right)P_k(k)\mathrm{d}k.\end{aligned}$$

One can easily show that the two integral terms in this strict relationship becomes negligible when $s\to\infty$. Under an additional condition that Eq. (S3.4) holds with $-\delta_l=-1-(\delta_k-1)/\gamma_1$,

$$\mathrm{P}(s|l=l_1)=\frac{\mathrm{P}(l=l_1,s)}{\mathrm{P}(l=l_1)}\sim\frac{1}{{l_1}^{(\alpha+\beta\gamma_1)/\gamma_1}}\tilde{P}_{s|l}\left(\frac{s}{{l_1}^{(\alpha+\beta\gamma_1)/\gamma_1}}\right)$$

at $l_1\to\infty$ and $s/{l_1}^{(\alpha+\beta\gamma_1)/\gamma_1}\to\infty$, where

$$\tilde{P}_{s|l}(\tilde{s})={l_0}^{(\alpha+\beta\gamma_1)/\gamma_1}\cdot\mathrm{P}\left(l=l_0,s={l_0}^{(\alpha+\beta\gamma_1)/\gamma_1}\cdot\tilde{s}\right).$$

Therefore, comparing this result with Eq. (S2.3), we have

$$\gamma_3=\frac{\alpha+\beta\gamma_1}{\gamma_1},\tag{S3.10}$$

for the upper tail of $s$ in a limited condition.

Here, we discuss the methods and results of our estimation of the scaling exponents in detail. First, we consider the rationales behind the estimations. Second, we check the consistency between the estimated scaling exponents with the mathematical relationships examined in Supplementary Text 3, in order to determine the thresholds that are used in the estimations. Third, we investigate the subtle changes of the scaling exponents with year and their relationships with GDP.

We first begin with the bivariate scaling relationships, formulated with Eqs. (S2.1–3) or (S3.1) and confirmed to be present in our data:

$$\mathrm{P}(x|y) = \tilde{P}_{x|y}(x/y^{\gamma})/y^{\gamma},$$

where $\mathrm{P}(x|y)$ is the probability density of $x$ conditional on $y$, $\tilde{P}_{x|y}$ is a probability density function and $\gamma$ is a positive constant. When a variable $\tilde{x}$ is defined as $\tilde{x} \equiv x/y^{\gamma}$, we have

$$\mathrm{P}(\tilde{x}|y) = \tilde{P}_{x|y}(\tilde{x}),$$

given that the probability density should satisfy the normalization $\int \mathrm{P}(\tilde{x}|y)\,\mathrm{d}\tilde{x} = 1$. The variable $\tilde{x}$ does not depend on the $y$-value and, thus, $\tilde{x}$ is independent of $y$.

This means that the exponent $\gamma$ could be estimated by finding the optimal value that makes the $\tilde{x}$ and $y$ the most independent of each other. One of the simplest indexes for measuring the dependence between stochastic variables is the Pearson's product-moment correlation coefficient. Therefore, we obtain $\hat{\gamma}$, the estimated value of $\gamma$, by

$$\hat{\gamma} = \arg\min_{\gamma}\left(\mathrm{Cor}\left[\log\left(\frac{x}{y^{\gamma}}\right),\ \log y\right]\right)^2. \tag{S4.1}$$

where $\mathrm{Cor}[\cdot,\ \cdot]$ means the correlation coefficient of the two terms. We apply the log-transformation to the raw data because the distribution of $x$ conditional on $y$ is heavy-tailed as shown in Fig. S4d–f. A few extreme values out of such heavy-tailed distributions could have a relatively high impact on the correlation coefficient compared to those from normal or exponential distribution as shown in Table S1.

This amounts to the linear least squares regression of $\log x$ against $\log y$. Indeed, when the correlation coefficient is zero, so is the covariance, and if we apply the transformations $x \leftarrow x/\bar{x}$ and $y \leftarrow y/\bar{y}$ where $\bar{x}$ and $\bar{y}$ represent the geometric mean of $x$ and $y$,

$$(N-1)\cdot\mathrm{Cov}\left[\log\left(\frac{x}{y^{\gamma}}\right),\ \log y\right] \equiv \sum_i \log y_i \cdot (\log x_i - \gamma \log y_i) = 0$$

or

$$\sum_i \log x_i \cdot \log y_i = \gamma \sum_i (\log y_i)^2, \tag{S4.2}$$

where $\mathrm{Cov}[\cdot,\ \cdot]$ means the covariance of the two, $N$ is the number of samples and $x_i$ and $y_i$ denotes the $i$-th sample of $x$ or $y$. Meanwhile, when the residual sum of squares is minimized,

$$\frac{\partial}{\partial\gamma}\sum_i (\log x_i - \gamma \log y_i)^2 = 0,$$

which is also satisfied by Eq. (S4.2).

Similar considerations are valid for the estimation of exponents in multi-variate scaling. Assuming Eq. (3),

$$\mathrm{P}(s|k,l) = \tilde{P}_{s|k,l}(s/k^{\alpha}l^{\beta})/k^{\alpha}l^{\beta},$$

and defining $\tilde{s} \equiv s/k^{\alpha}l^{\beta}$, $\mathrm{P}(\tilde{s}|k,l) = \tilde{P}_{s|k,l}(\tilde{s})$ follows. Therefore, $\alpha$ and $\beta$ could be estimated with

$$(\hat{\alpha},\hat{\beta}) = \underset{\alpha,\beta}{\arg\min}\left[\left(\mathrm{Cor}\left[\log\left(\frac{s}{k^{\alpha}l^{\beta}}\right),\ \log k\right]\right)^2 + \left(\mathrm{Cor}\left[\log\left(\frac{s}{k^{\alpha}l^{\beta}}\right),\ \log l\right]\right)^2\right]. \quad \text{(S4.3)}$$

When the correlations are zero so that the right hand side of Eq. (S4.3) is minimal, and when we apply the transformations $s \leftarrow s/\bar{s}$, $k \leftarrow k/\bar{k}$ and $l \leftarrow l/\bar{l}$, where $\bar{x}$ denotes the geometric mean of a variable $x$,

$$\sum_i (\log s_i - \alpha \log k_i - \beta \log l_i) \cdot \log k_i = \sum_i (\log s_i - \alpha \log k_i - \beta \log l_i) \cdot \log l_i = 0,$$

where $k_i$, $l_i$ and $s_i$ denotes the $i$-th sample of $k$, $l$ or $s$. In this condition, we can see that

$$\frac{\partial}{\partial \alpha}\sum_i (\log s_i - \alpha \log k_i - \beta \log l_i)^2 = 0;\quad \frac{\partial}{\partial \beta}\sum_i (\log s_i - \alpha \log k_i - \beta \log l_i)^2 = 0. \quad \text{(S4.4)}$$

Therefore, the estimation in Eq. (S4.3) is equated to the linear least squares regression of $\log s$ against $\log k$ and $\log l$, without the interaction term.

Although it is more formal to orthogonalize explanatory variables in the regression analysis, the method presented above gives a result equivalent to the orthogonalized version. Let us consider the regression of $\log s$ against $\log k$ and $\log[l/k^{\gamma_1}]$, where $\gamma_1$ is a constant determined empirically ($\gamma_1 \sim 1.0$ as later shown in as shown in Fig. S5c). The variables are again normalized with the transformation $x \leftarrow x/\bar{x}$, where $\bar{x}$ represents the geometric mean of a variable $x$. Here, the exponents, $\alpha'$ and $\beta'$, are intended to fulfill the multi-variate scaling $s \propto k^{\alpha'}(l/k^{\gamma_1})^{\beta'}$ and thus estimated as

$$(\hat{\alpha}',\hat{\beta}') = \underset{\alpha',\ \beta'}{\arg\min}\left[\mathrm{Cor}\left[\log\left(\frac{s}{k^{\alpha'}(l/k^{\gamma_1})^{\beta'}}\right),\ \log k\right]^2 + \mathrm{Cor}\left[\log\left(\frac{s}{k^{\alpha'}(l/k^{\gamma_1})^{\beta'}}\right),\ \log(l/k^{\gamma_1})\right]^2\right].$$

When the correlations are zero,

$$\sum_i \big(\log s_i - \alpha' \log k_i - \beta'(\log l_i - \gamma_1 \log k_i)\big) \cdot \log k_i = 0; \quad \text{(S4.5)}$$

$$\sum_i \big(\log s_i - \alpha' \log k_i - \beta'(\log l_i - \gamma_1 \log k_i)\big) \cdot (\log l_i - \gamma_1 \log k_i) = 0. \quad \text{(S4.6)}$$

Adding Eq. (S4.6) to Eq. (S4.5) multiplied by $\gamma_1$, we have

$$\sum_i \big(\log s_i - \alpha' \log k_i - \beta'(\log l_i - \gamma_1 \log k_i)\big) \cdot \log l_i = 0. \quad \text{(S4.7)}$$

Equations (S4.5) and (S4.7) is met with $\alpha' = \alpha + \beta\gamma_1$ and $\beta' = \beta$ when Eq. (S4.4) holds. Therefore, the estimated value of exponents in a formal regression analysis can be derived from the regression with the explanatory variables not orthogonalized. Note that $\alpha'$ is just the mathematically expected value of $\gamma_2$ as shown in Eq. (S3.9).

Although the linear regressions could give the estimations of scaling exponents in principle, we should consider what data to exclude from the analysis. This is because the scaling relations do not perfectly describe the data for all ranges of variables. For example, we can see some deviations from the scaling relations especially for the number of trading partners $k$ and the employee number $l$ less than 10 (Figs. 2a and S4a–c). Since firms of smaller size dominate the data (Fig. S2), their deviation from the scaling should heavily affect the estimation. Indeed, without any data exclusion from the compiled data, there is a considerable gap between the direct and indirect estimations of $\delta_l$ (the power-law exponent of $l$ distribution). Whereas we see that $\delta_l \approx 2.2$ from Fig. S2b, $\delta_l \approx 2.7$ is expected from Eqs. (S3.4) and (S3.5), since $\gamma_1 \approx 0.75$ (Fig. S5a), $\delta_{l|k} \approx 2.7$ (Fig. S4d) and $\delta_k \approx 2.2$ (Fig. S2a). To ensure the consistency between the exponents, $\gamma_1 \approx 1.0$ should hold. Additionally, there is a clear difference between the expected value of $\gamma_3$ (dashed purple line) from Eq. (S3.10) and the value of direct estimation (solid purple line) as shown in Fig. S5a.

To obtain a consistent set of estimates that does not contradict the mathematical relations mentioned in Supplementary Text 3, we try two thresholds, 10 and 100. If the 'explanatory' variables in the right hand side in Eq. (2) or Eqs. (S2.4–6) take a value under the threshold, we neglect the datum. The results are shown in Fig. S5b for the threshold 10 and 5c for 100. We see that $\gamma_1$ nearly becomes 1.0 and the direct and indirect estimates of $\gamma_3$ agree to each other only when the threshold is set at 100. This suggests that the threshold should be no less than 100 for $k$ and $l$. For the sake of sample size, we employ the threshold value of 100. The sample sizes before and after the threshold is applied are shown in Fig. S5d.

We determine the scaling exponents for every year to assure the stability of our results. Yearly estimation of the exponents is shown in Fig. S5c. The slow fluctuations of estimated $\alpha$ (black line) and $\beta$ (red line) are noticeable. However, we need an uncertainty measure to judge whether the fluctuations are meaningful.

Despite our use of linear regression, the estimation of uncertainty needs a nonparametric method, since the 'error terms' (Fig. S4d–f) are not normally distributed. To this end, we perform the bootstrap method [7] to get the CI (confidence intervals). Resampling is done 10,000 times and the resampling size is identical to the sample size. The 95% confidence intervals are determined as the 2.5- and 97.5-percentiles of the bootstrap distribution.

Although the changes are not radical and the inequality $\alpha < \beta$ is invariably met, as shown in Fig. 4, The exponents $\alpha$ and $\beta$ become smaller and larger respectively in the 2000–2005 period compared to the 2013–2015 period. The difference is 'significant' in the loose sense that the 95% confidence intervals are not overlapping. It is also clear that $\alpha$ and $\beta$ are negatively correlated, which is expected from Eq. (S3.9) and relatively constant $\gamma_1$ and $\gamma_2$ (Fig. S5c). This implies that the only variants in the system at this level of coarse-grained observation are the values of $\alpha$ and $\beta$, considering the relative invariability of $\gamma_1$, $\gamma_2$ and $\gamma_3$ and distributional functions (Figs. 2f and S5c).

It is intriguing to see that $\alpha$ and $\beta$ respectively seem counter- and pro-cyclical: i.e. it is apparently positively or negatively correlated to the nominal GDP of the country [8], as indicated in Figs. S6a and S6b. GDP is selected here because its cycle of fluctuation is longer compared to other indices of the economic climate, such

as Indexes of Business Conditions reported by Cabinet Office, Government of Japan [9]. A closer inspection reveals that $\alpha$ is enlarged when the nominal GDP decreases (Fig. S6a) and that $\beta$ goes down almost simultaneously with GDP while its increase is delayed with respect to GDP expansion (Fig. S6b). However, we could not rule out the possibility that this is a mere coincidence, since the dataset covers only slightly more than one cycle. Considering the fact that the cycle is about twenty years long, it might need one more decade or a dataset from another country to verify this trend.

We furthermore calculate the cross-correlation between GDP and the exponents to evaluate the delay quantitatively. The normalized cross correlation $\mathrm{CC}_\tau[x, y]$ is here defined by the Pearson's correlation coefficient applied to lagged time-series data $x(t)$ and $y(t+\tau)$ defined for discrete time $t_0 \le t \;(\in \mathbb{Z}) \le t_{\mathrm{end}}$:

$$\mathrm{CC}_\tau[x, y] \equiv \frac{1}{N-1}\sum_{T_\tau} \tilde{x}(t)\tilde{y}(t+\tau) \Bigg/ \sqrt{\frac{1}{N-1}\sum_{T_\tau} \tilde{x}(t)^2}\sqrt{\frac{1}{N-1}\sum_{T_\tau} \tilde{y}(t+\tau)^2},$$

where $T_\tau \equiv \{t \in \mathbb{Z} \mid t_0 + \tau \le t \le t_{\mathrm{end}} + \tau\}$, $N$ is the length of the time-series (i.e. the number of elements in the truncated set $T_\tau$) and

$$\tilde{x}(t) \equiv y(t) - \frac{1}{N}\sum_{T_\tau} y(t) \text{ and } \tilde{y}(t) \equiv y(t) - \frac{1}{N}\sum_{T_\tau} y(t).$$

We plot $\mathrm{CC}_\tau[\mathrm{GDP}, \hat{\alpha}]$ and $\mathrm{CC}_\tau[\mathrm{GDP}, \hat{\beta}]$ against $\tau$ in Fig. S6c, and see that both peaks at $\tau = 1$ (negatively and positively, respectively), with Pearson correlation coefficient as high as –0.59 and 0.58. To add, the second highest peak is present in both cross correlation series, probably reflecting the fact that the extent of delay in exponent changes is different for GDP increase and decrease. Note that the reversal of sign at $\tau$ value far from 0 is the artefact of the time window that covers only slightly more than one economic cycle. The result suggests that the scaling exponents are affected by GDP of the previous year on average. We suspect that some parameters in inter-firm trades are mechanistically affected by GDP. However, we have no further support for this statement at the present study.

In this note, we assess the generality of the results represented in Fig. 5 for firms of different sizes. Fig. 5 shows that Group 2 firms (with an employee growth by a factor over 1.5) outperform Group 1 firms (with a trading partnership growth by a factor over 1.5) in sales growth on average when the size vector in the initial year is controlled for. However, in the main text, we only examine the case of the number of trading partners $k \sim 10$. Here we check the validity of our claim in other cases.

We first compare Group 2 against Group 1 for different sets of firms on the scaling line (Fig. 3a) with the same setup as in the main text. More specifically, the following procedures are applied to our data. First, a point on the scaling line is determined from a value of $k$, ranging from $10^0$ to $10^4$, with Eq. (S6.1). Firms' Euclidean distance $d_{\log}$ from this point in log-transformed scales (Eq. (5)) is used to obtain a set of firms that are

located closely around the point (i.e. $d_{\log} < \log[10^{1/8}]$) in the initial year $t$–1. The firms are searched over the entire data, but the initial year ranges from 1994 only to 2013 so that we can trace the sales change in the following year $t$+1. If the sample size does not reach 1,000, the threshold of $d_{\log}$ is enlarged until there are equal to or more than 1,000 samples. Then, we determine three mutually exclusive sets of firms from these samples, namely (i) 'Control' firms whose yearly changes in both the number of trading partners $k$ and employee number $l$ are within ±20%, (ii) 'Group 1' firms which increase the number of trading partners $k$ by over a factor of 1.5 in a year but keep their change in employee number $l$ within ±20% and (iii) 'Group 2' firms which grow in $l$ by over a factor of 1.5 in a year but keep their $k$ change within ±20% in the same period. This ensures that the correlation between $g_k$ (annual $k$ growth) and $g_l$ (annual $l$ growth), which is already weak (SFig. S8), does not affect the difference between these groups. Averages of the log-transformed sales growth in the same year ($\log[s(t)/s(t-1)]$) and in the following year ($\log[s(t+1)/s(t)]$) are calculated for each group of firms, and the uncertainty of the value is indicated by the 95% confidence interval determined by the bootstrap method [7], where 2.5- and 97.5-percentiles in the resampling distribution is obtained from 10,000 resamplings.

It is evident that the average sales growth of Group 2 firms is higher compared to that of Group 1 firms when the firm size in the number of trading partners $k$ is smaller than 30, as is shown in Fig. S7a and b. This is true both for the 'coinciding' sales growth in the year $t$ (Fig. S7a) and for the 'following' one in the year $t$+1 (Fig. S7b). Additionally, the average growth of Group 1 or Group 2 firms is almost always above the level of Control firms, suggesting that the growth either in $k$ or in $l$ has a positive effect on the sales growth.

However, the difference between Group 1 and 2 is hard to see for larger firms, largely because of the fewer sample sizes. Also note that the size fluctuation is smaller for larger firms [4,10–13], and the larger the firm is, the rarer is the ratio of firms that experience a size growth higher than 50%. The weak but higher correlation between $k$ and $l$ growth in large firms compared to the small firms (Fig. S8) further reduces the number of firms included in the high-growth groups.

To address this problem, we also relax the definition of Group 1 and 2, allowing firms which grow in $k$ or $l$ by over a factor of 1.2 (instead of 1.5) to enter the groups. The results are shown in Fig. S7c and d. They also support the difference of sales growth between the two groups when the initial $k$ of the firms is smaller than 30, but it seems that growth in the number of trading partners sometimes has more positive effect on sales growth in the same year compared to employee growth when the initial $k$ is larger than 100. It is hard to conclude, however, as again the sample size is still small. For example, even in this setting, we have only 14 and 13 firms for Group 1 and 2 when the initial firm size is set to be $k \sim 10^3$. Also note that a high risk of false positives is present, where a significant effect is detected from the sample data although no such effect exist in experimental situations, since multiple comparisons are performed here for sets of firms of different sizes.

To sum, Group 2 firms (with a large employee growth) has higher sales growth compared to Group 1 firms (with a large growth in the number of trading partners), at least when the firms are small- or medium-sized ($k < 30$). Group 1 and Group 2 firms are both likely to outperform Control firms with small changes in employee size or trading partnership. However, it is unclear whether Group 2 always attain higher sales growth on average

compared to Group 1 when the firms are large.

This note provides a detailed explanation of the methods and results regarding the evolutionary flow diagrams. First, we explain how to determine the absolute position of the 'scaling line' shown in the diagrams. Second, we describe the methodology whereby we render streamlines indicating the flow. Third, we describe the results in more detail than in the main text, showing slices covering entire ranges of the 3-dimensional vector space.

We define the 'scaling line' in accordance with Eqs. (2) and (S2.4). Taking the median of their right hand side, we have

$$\log l = \gamma_1 \log k + \langle \varepsilon_{l|k} \rangle_{0.5} \quad \text{and} \quad \log s = \alpha \log k + \beta \log l + \langle \varepsilon_{s|k,l} \rangle_{0.5} \,, \tag{S6.1}$$

which can be interpreted as planes in the 3-dimensional space. We regard the line of intersection of these planes as the central line of scaling. Although the line should be determined only from the bivariate scaling relations in principle, there would be difficulty since there does not always exist a 3-dimensional line such that different lines on three different planes are just the projections of the 3-d line to the planes. We use the median rather than with the average here, because the distribution of $l$ conditional on $k$, $\tilde{P}_{l|k}$ (Fig. S4d), or of $s$ conditional on both $k$ and $l$, $\tilde{P}_{s|k,l}$ (Fig. 2b) is heavy-tailed and the average does not give an intuitive representative value. We thus compute the medians of $\log l - \gamma_1 \log k$ and $\log s - \alpha \log k - \beta \log l$ as the intercept of the planes, where the sample of $k$ (for the former) or both $k$ and $l$ (for the latter) is confined above the threshold 100. The values of $\alpha$, $\beta$ and $\gamma_1$ used in the calculation are estimated in the same way as in Methods section, except that the source data are aggregated regardless of the year.

We rendered the streamlines in Figs. 6 and S9, exploiting the method developed elsewhere [14] in order to render a 2-dimensional diagram which is visibly easy to interpret. In summary, it follows two steps: (i) placing some points randomly on the plane and drawing streamlines that pass through them, and (ii) repeatedly comparing the original image with a randomly modified one and selecting the one in which the streamlines are placed more homogeneously. Random modifications include inserting, deleting, lengthening, shortening and (almost) parallel moving of a streamline and combining of two. The measure of homogeneity for a set of placed streamlines is defined with a blurred image of them.

We render the individual streamlines by the 4th order Runge-Kutta method. For the purpose of reducing the computational power required, we apply the transformation below to the original vector field:

$$\boldsymbol{g}(k,l,s) \leftarrow \frac{\boldsymbol{g}(k,l,s)}{|\boldsymbol{g}(k,l,s)|^c} \,,$$

where $g(k,l,s)$ in the right hand side represents the 3-dimensional vector of average log-transformed growths at a point in the vector space, estimated as in Methods section, and $0 < c < 1$ the degree of 'acceleration'. In this transformation, the streamlines ideally remain the same, since the direction in which an average firm of the size vector proceeds does not change at any point. It, however, accelerates the iteration when the speed is nearly

0, thus drastically reduces the computational needs. We set $c = 0.7$, considering the trade-off between the computational power reduced and precision of the drawing near the equilibrium point.

Some minor adjustments applies to the method. One is the omission of re-calculation of streamlines. In the original method, one should render the streamlines from scratch every time the modification is performed. This is not computationally feasible in our case, due to the fact that the drawing of a streamline need a substantial computational power. To apply the original methodology of streamline selection in this situation, we obtain 400 lines in advance and assign numbers to them such that a line to which a number is assigned is closer to the lines of the adjacent numbers than to other ones. Another adjustment in the algorithm is that the random combining is not allowed here. This serves to avoid combining streamlines of different orientations.

We exhibit all the resulting evolutionary flow diagrams for a variety of slicing planes in Fig. S9. The vector space is sliced with planes of a constant $k$ (trading partners number) that ranges from 1 to $10^4$ in Fig. S9a–e; a constant $l$ (employees number) that ranges from 1 to $10^4$ in 8f–j; a constant $s$ (annual sales in million yen) that ranges from 1 to $10^6$ in 8k–q.

We notice several remarkable aspects. The first one is that firms generally flow towards the scaling surface (see Fig. 2a for data of year 2014 and Fig. 6 for aggregated data). The contours indicating the surface are marked by yellow lines in the figures. Although the sales growth is not exactly zero at all the points in the scaling surface, this might well occur as a result of stochasticity and uncertainty. The fact lends credibility to the observation, that the trend of near-zero growth on the scaling surface is more obvious at the center of yellow contours and at medium $s$-levels than elsewhere, as the sample density is larger in these zones.

Secondly, we note the ubiquitous flow toward the scaling (red) point for slice with $l$ in Fig. S9f–j or with $s$ in Fig. S9k–q. Additionally, the speed of flow is almost zero around the red point, indicating the fact that firms hardly move on average once they reach this point. It follows that the scaling line is an attractor if we regard the system as a dynamical system, where the firm development is determined only by the average flow and has no stochasticity. Note that this might not be the case for the largest firms: firms with the highest number of employees $l$ ($> 10^4$) with $k > 10^3$ and $s > 10^5$ tend to decrease their employees, and seem more stable at a smaller $l$. If this is true, it might be related to the seeming plateau of $s$ at the highest $l$ (Fig. S4c). However, the degree for which this is true is a matter of question, as the estimates of growth rates would be inaccurate there.

Third, as visible in slices with a constant sales $s$ in Fig. S9k–q, increasing of trading partners does not have so positive effect on the sales growth rate as the employee increase. It even negatively affect the sales growth when sales is low (Fig. S9k and l).

We also show contour plots of firm exit rates for a variety of slicing planes in Fig. S10. The space is sliced with the same planes as in Fig. S9. We can see two phases in the figures. First, when the firms are over the medium size (i.e. $k \geq 10$, $l \geq 10$ or $s \geq 10^3$), the exit rate is generally higher at locations far from the scaling (red) point than at the vicinity of it, although it is not homogeneously high. In contrast, in the case where the sales is very low (i.e. $s < 10^2$, Fig. S10k and l), where no $k$ or $l$ value larger than 1 is possibly on scaling, lower exit rate coincides with more trading partners $k$ and less employees $l$. Note that the placement of background colors in Fig.

S10k and l are similar to that in Fig. 9k and l. This suggest that the two phases mentioned in this paragraph also regulate some aspects of growth rates.

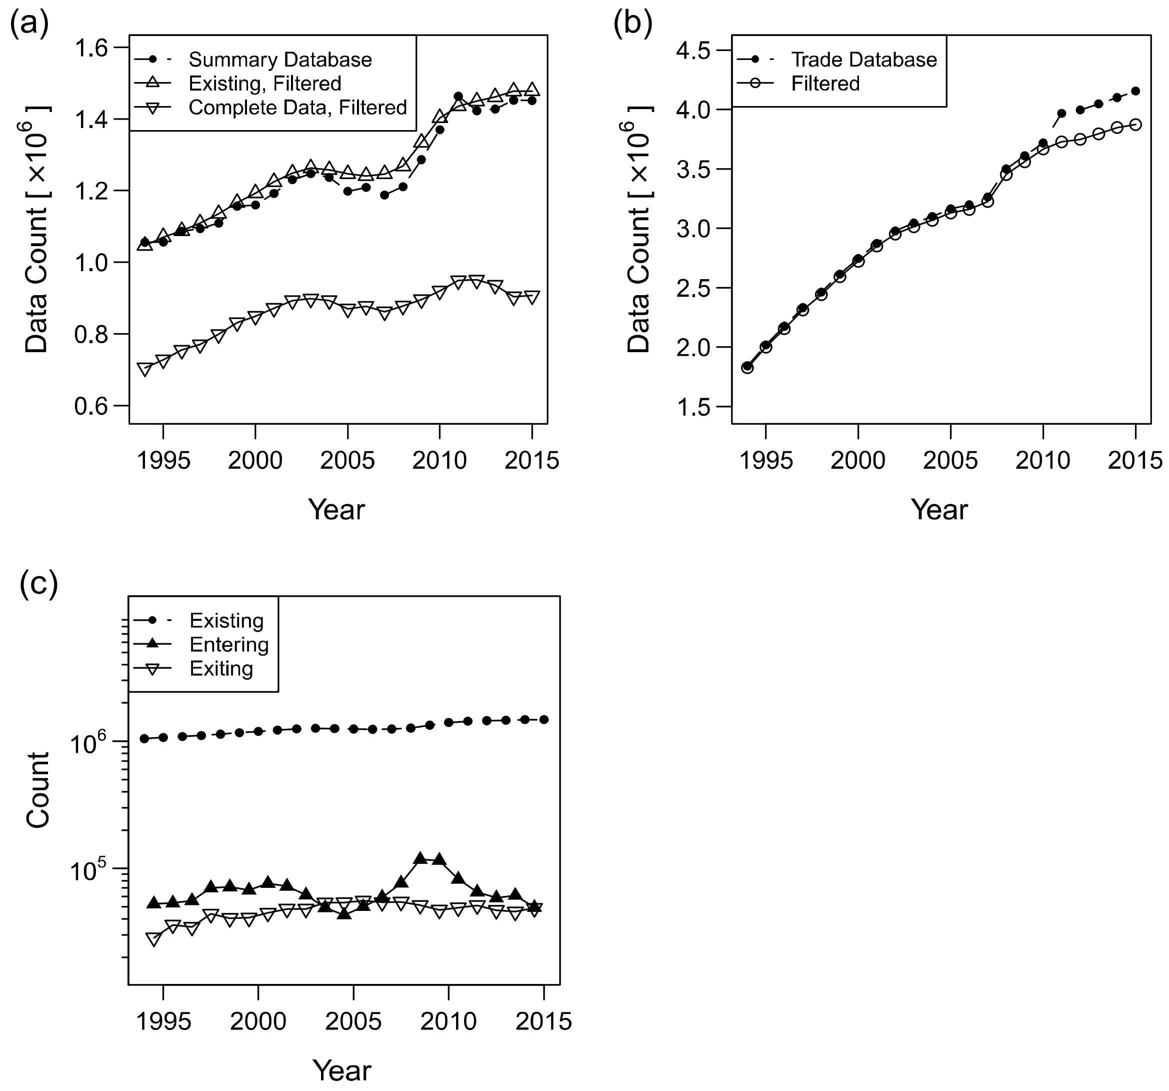


**Figure S1. Change of data amount through the period 1994–2015.** (**a**) The data amount of the original summary database (dashed line and black dots), number of existing firms after the filtering and integration with network data (upward triangle) and firms with data of all the three variables (downward triangle). (**b**) The data amount (number of links) of the original trade database (dots) and the after the filtering (circles). (**c**) The number of appearing (upward triangle) and disappearing (downward triangle) firms. The number of existing firms (dots) are plotted for the sake of comparison. Note that the vertical axis is in logarithmic scale.

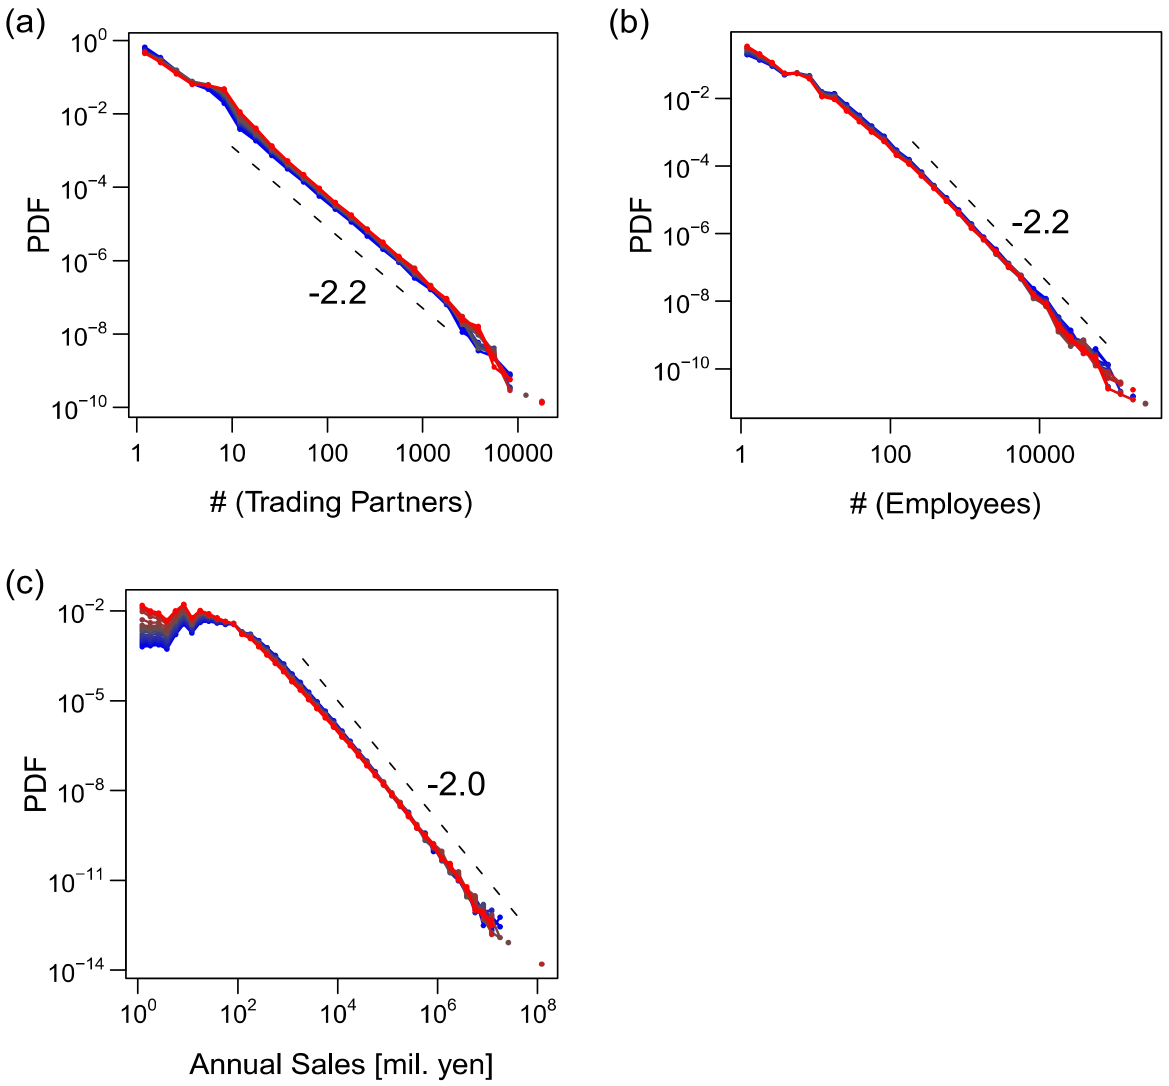


**Figure S2. Probability distribution function (PDF) of the size variables through the period 1994-2015.** The figures are plotted in log-log scales. Blue to red gradient of the color indicate the direction from old to new data. (**a**) Trading partners number. (**b**) Employee number. (**c**) Annual sales in million yen.

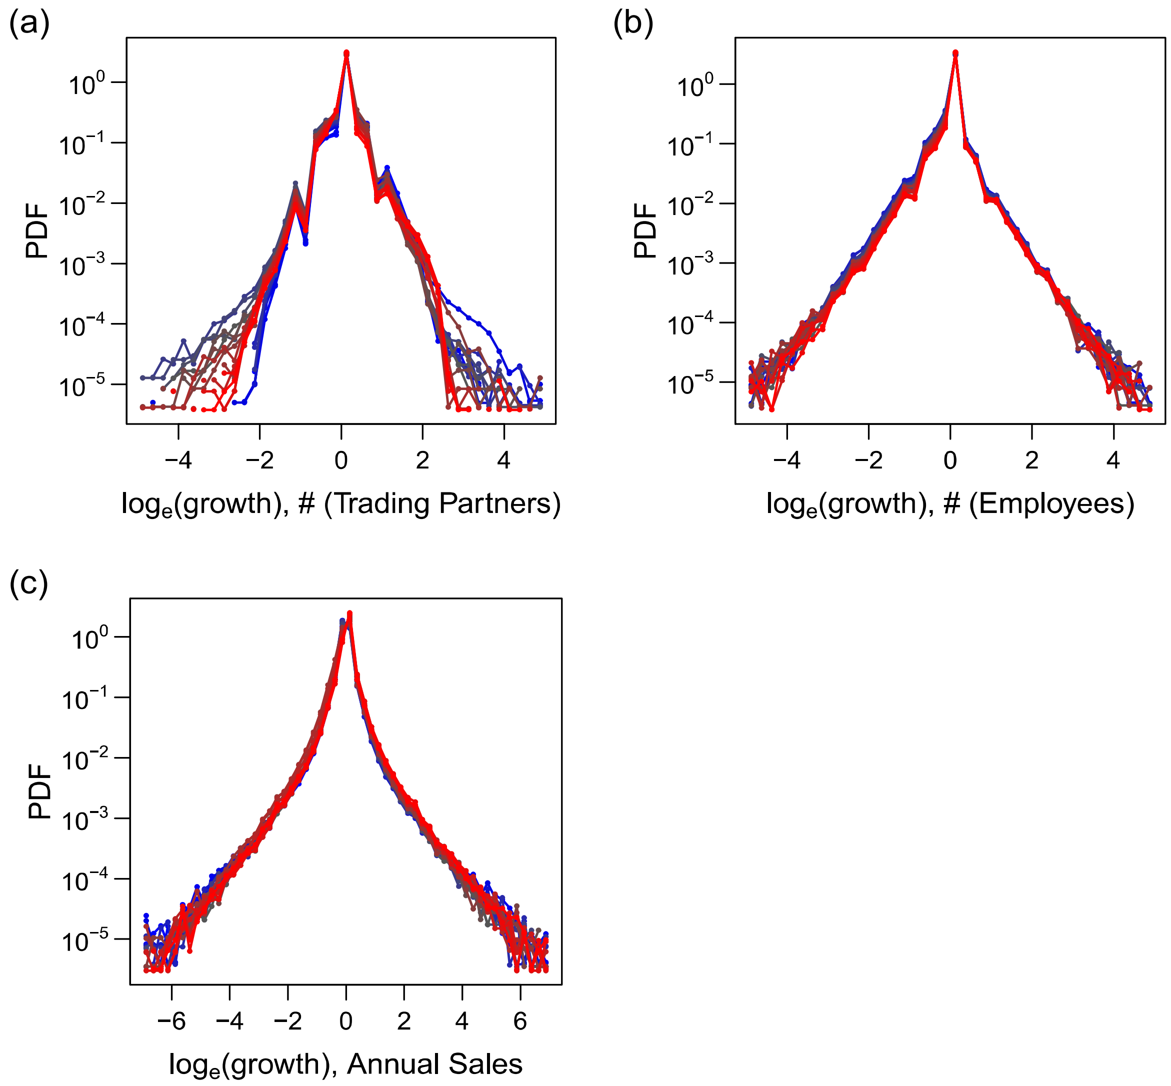


**Figure S3. Probability distribution function (PDF) of the growth rate of size variables transformed by natural logarithm through the period 1994–2015.** Growth rate is defined as the ratio of a value at a given year to that at the previous year. The distribution is not conditional on another variable. Note that the vertical axis is plotted in logarithmic scale. Blue to red gradient of the color indicate the direction from old to new data. (**a**) Growth rate of trading partners number. The zigzagged form at the center is due to the fact that the number of trading partners are integer, and a very large fraction of firms has only a few trading partners (Fig. S2a). (**b**) Growth rate of employee number. (**c**) Growth rate of annual sales in million yen.

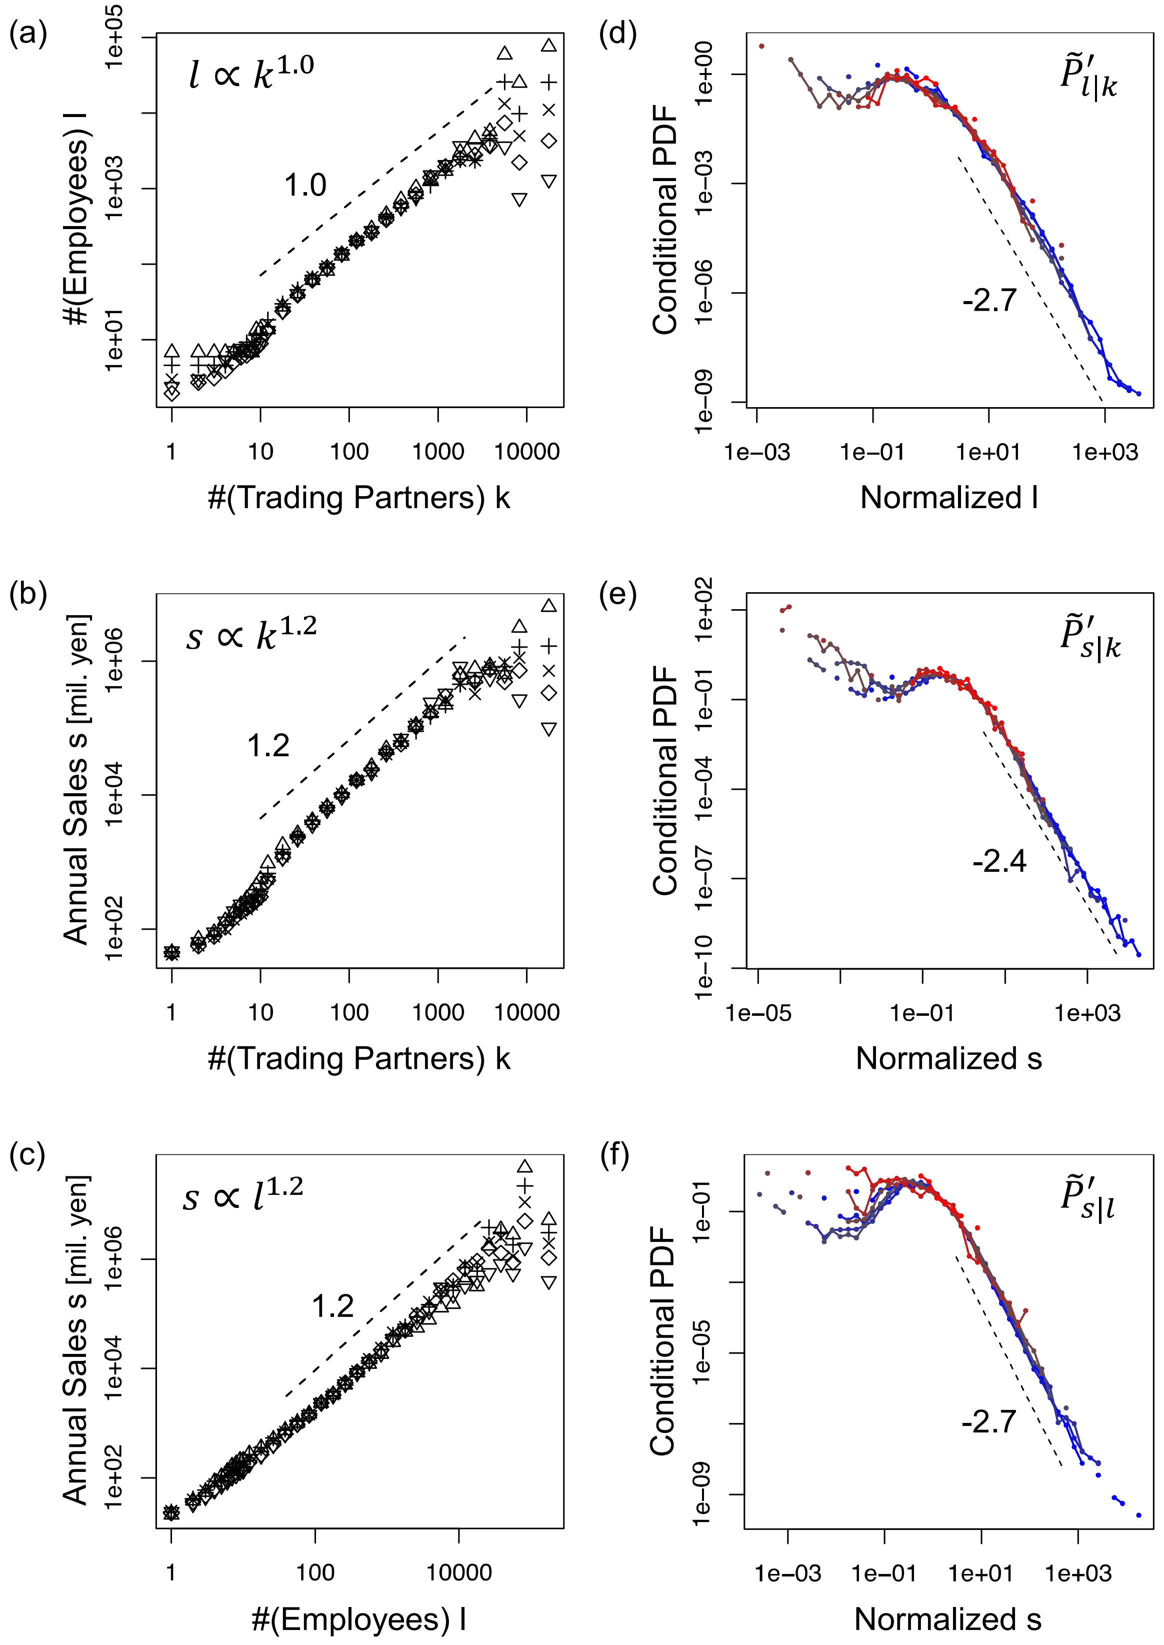

(a)
$l \propto k^{1.0}$
1.0
#(Employees) l
#(Trading Partners) k
(b)
$s \propto k^{1.2}$
1.2
Annual Sales s [mil. yen]
#(Trading Partners) k
(c)
$s \propto l^{1.2}$
1.2
Annual Sales s [mil. yen]
#(Employees) l
(d)
$\tilde{P}'_{l|k}$
-2.7
Conditional PDF
Normalized l
(e)
$\tilde{P}'_{s|k}$
-2.4
Conditional PDF
Normalized s
(f)
$\tilde{P}'_{s|l}$
-2.7
Conditional PDF
Normalized s

**Figure S4. Scaling relations between pairs of size variables.** The variables are the number of trading partners $k$, the number of employees $l$ and annual sales in million yen $s$. All the data used in the figures are for 2014. (**a–c**) The 0.95(▽), 0.75(+), 0.5(×), 0.25(◇) and 0.05(△) quantiles of conditional distribution of $l$ or $s$ (vertical axis) are plotted against another variable $k$ or $l$ (horizontal axis) in a log-log scale. The variable of horizontal axis is divided into intervals of identical lengths in log scale (6 segments per a 10-fold interval) for $k$ and $l$ >10 and of a unity in linear scale for $k$ and $l$ ≤10. Quantiles other than those of $q$ = 0.5 (i.e. medians) are plotted with horizontal shift, so that all the curves pass through a point whose $x$-axis is slightly more than 100. (**d–f**) The probability distributions (PDF) of $l$ or $s$ conditional on $k$ or $l$ (namely, $\mathrm{P}(l|k)$, $\mathrm{P}(s|k)$ and $\mathrm{P}(s|l)$), normalized by their conditional medians, are plotted in log-log scale. Conditional distributions are obtained for intervals of the 'explanatory' variable ($k$ or $l$), where the entire range (a unity to the maximum of the variable) is evenly divided logarithmically into 8 segments. Color gradient of blue to red of the points and curves indicates low to high values of the 'explanatory' variable.

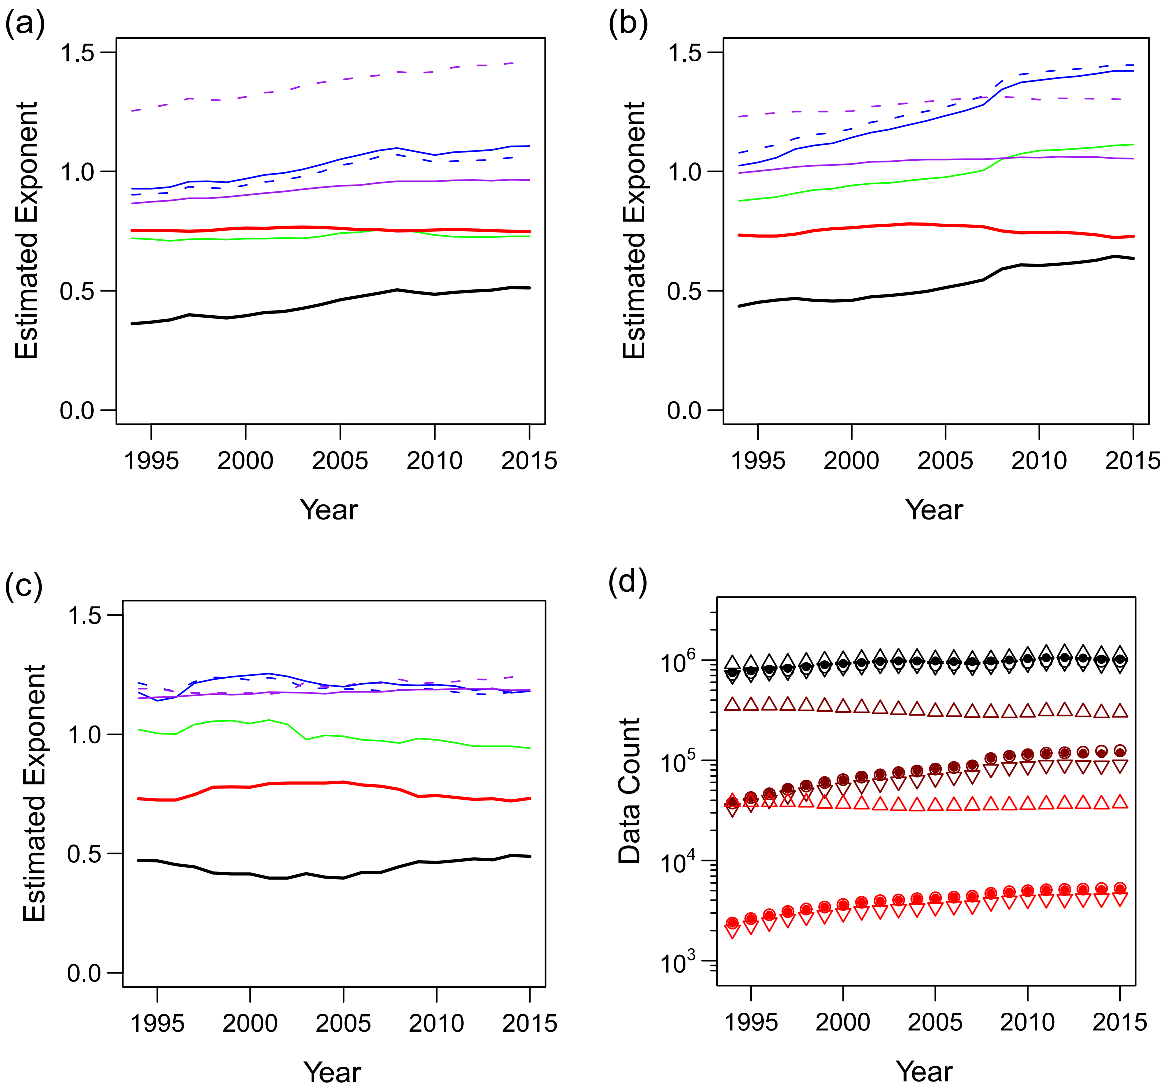


**Figure S5. Estimated exponents of the scaling relationships through the period 1994–2015.** The exponents of $l \propto k^{\gamma_1}$ (green), $s \propto k^{\gamma_2}$ (blue), $s \propto l^{\gamma_3}$ (purple) and $\alpha$ (black) and $\beta$ (red) in $s \propto k^{\alpha} l^{\beta}$ are plotted. Additionally, the expected value of $\gamma_2$ and $\gamma_3$ derived mathematically from $\alpha$, $\beta$ and $\gamma_1$ in case of perfect scaling (Supplementary Text 2, Eqs. (S2.9) and (S2.10)) are juxtaposed (dashed line in blue and purple). (**a**) All the available data is used to estimate the exponents. (**b**) Used only the data where the 'explanatory' variable is larger than 10. (**c**) Used only the data where the 'explanatory' variable is larger than 100. (**d**) Plot of the size of samples from which the exponents are estimated against the year. Black, brown and red points indicate the threshold 0 (no exclusion), 10 and 100, corresponding to panel (a), (b) and (c). Hollow (○) and filled (●) circles, upward (△) and downward (▽) triangles respectively represent the scaling of *l* vs. *k*, *s* vs. *k*, *s* vs. *l* and *s* vs. *k* and *l*.

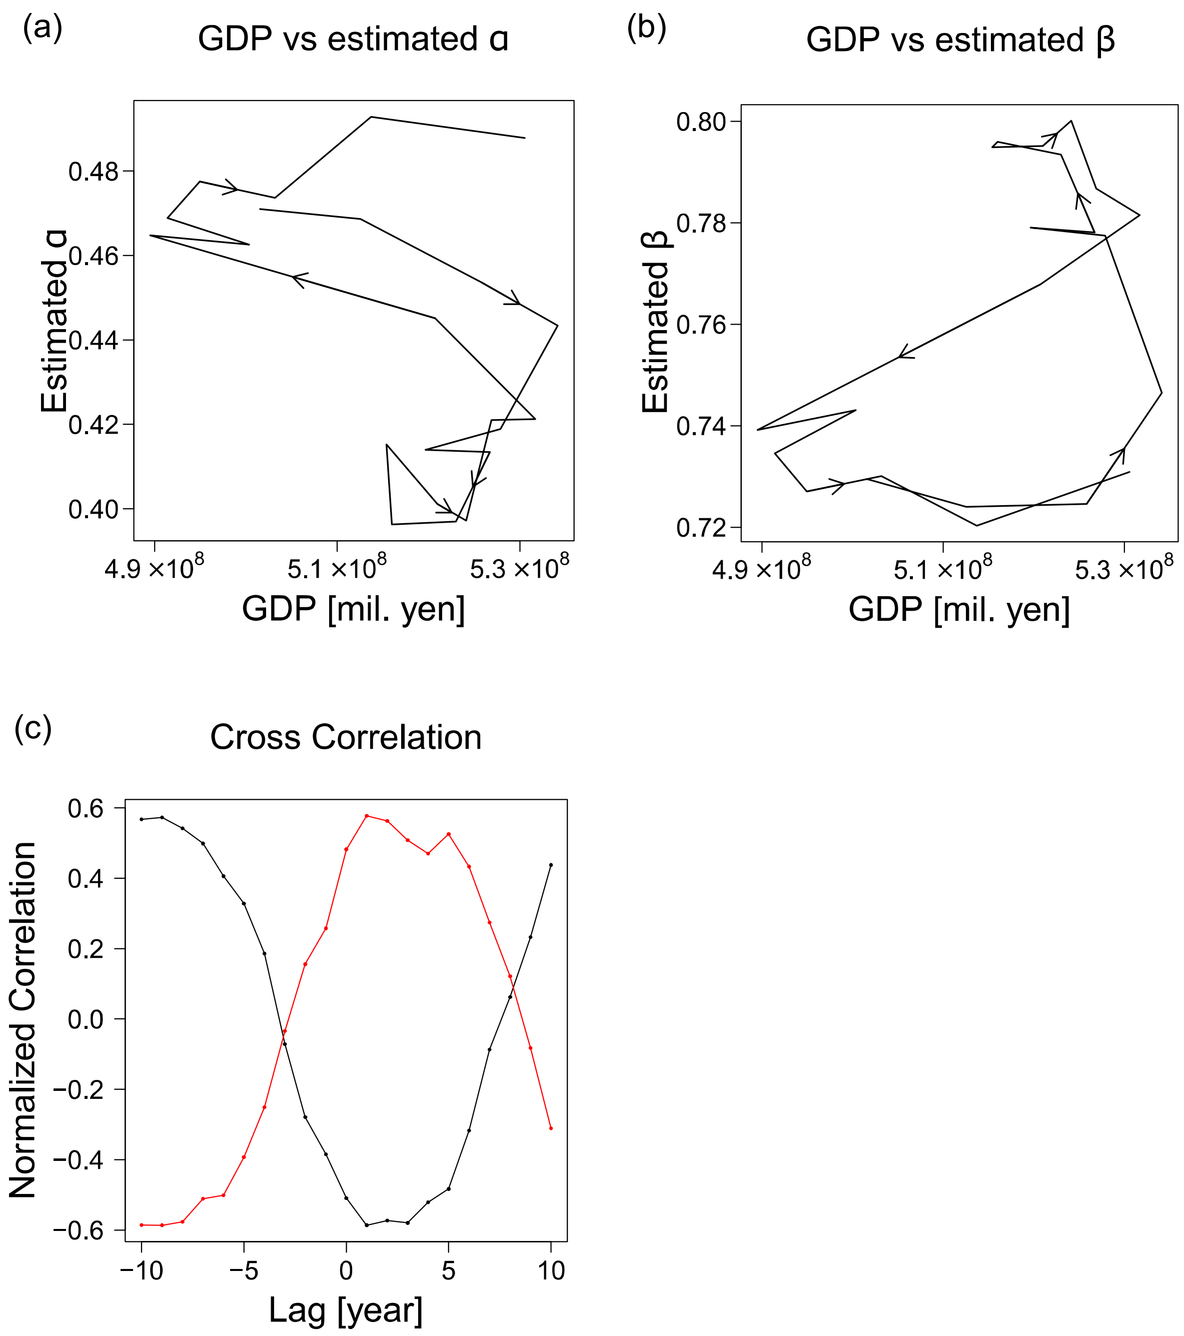


**Figure S6. Estimated exponents $\alpha$ (for the number of trading partners $k$) and $\beta$ (for the number of employees $l$) with the country's nominal GDP for different years in 1994–2015.** The arrows indicate the time evolution. (**a**) The estimated $\alpha$ against the GDP. (**b**) The estimated $\beta$ against the GDP. (**c**) Cross correlations between Nominal GDP and $\alpha$ or $\beta$ are plotted against the time lag.

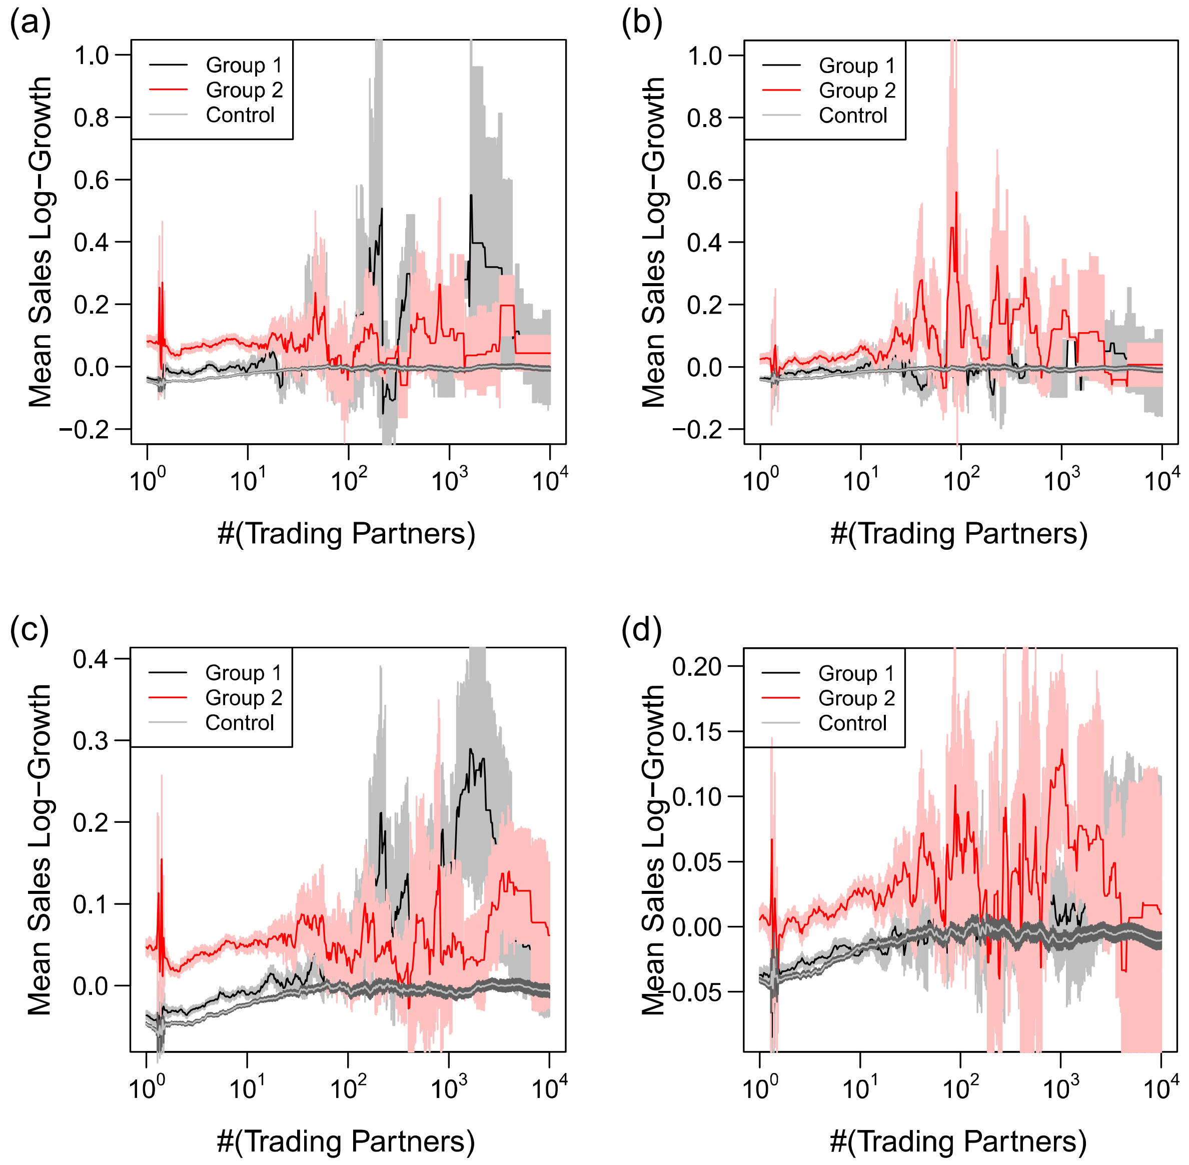


**Figure S7. Average log-transformed growth rate of firms in Group 1 (black), Group 2 (red) and Control group (light grey) against the initial firm size.** The colors around the line (grey for Group 1, pink for Group 2 and dark grey for Control) indicate 95% confidence intervals. The firm are sampled from around the scaling line. (**a–b**) Plot of average log-transformed sales growth of the same year (panel (a)) or the following year (panel (b)) against the firm size. Firms are included into Group 1 or 2 by over 50% growth in the number of trading partners or in employee number. (**c–d**) Plot of average log-transformed sales growth of the same year (panel (c)) or the following year (panel (d)) against the firm size. Firms are included into Group 1 or 2 by over 20% growth in the number of trading partners or in employee number.

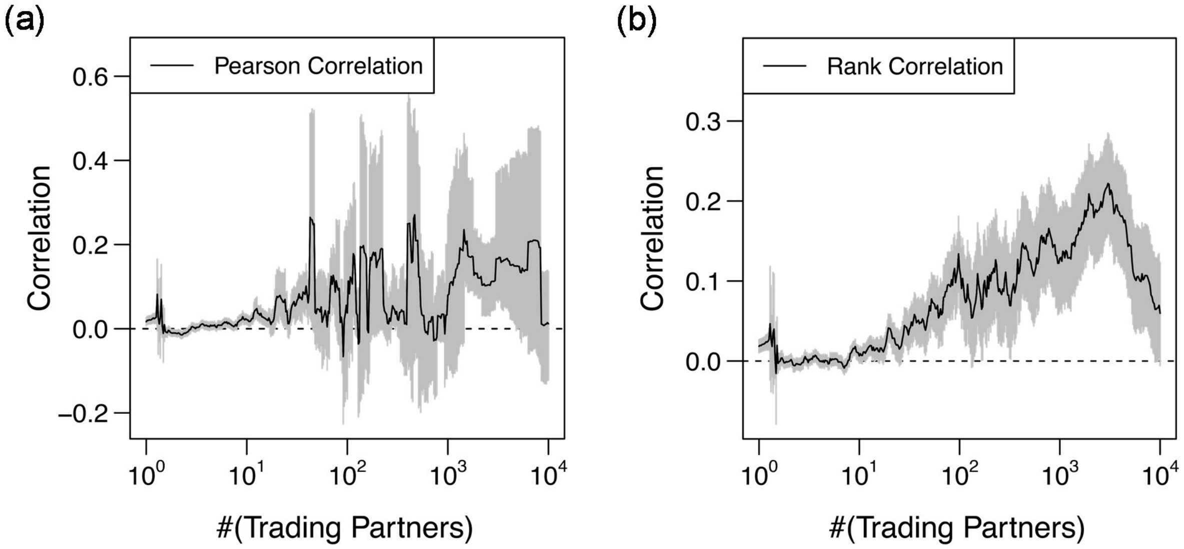


**Figure S8. Correlation coefficients between annual growth in trading partners and employees.** The central black curve is the estimated, while the grey bandwidth indicates the 95% confidence interval calculated by the bootstrapping method with 10,000 resamplings. (**a**) Plot of the Pearson correlation coefficient between the growth rates of employees and trading partners against the firm size. (**b**) Plot of the Spearman's rank correlation coefficient between the growth rates of employees and trading partners against the firm size.

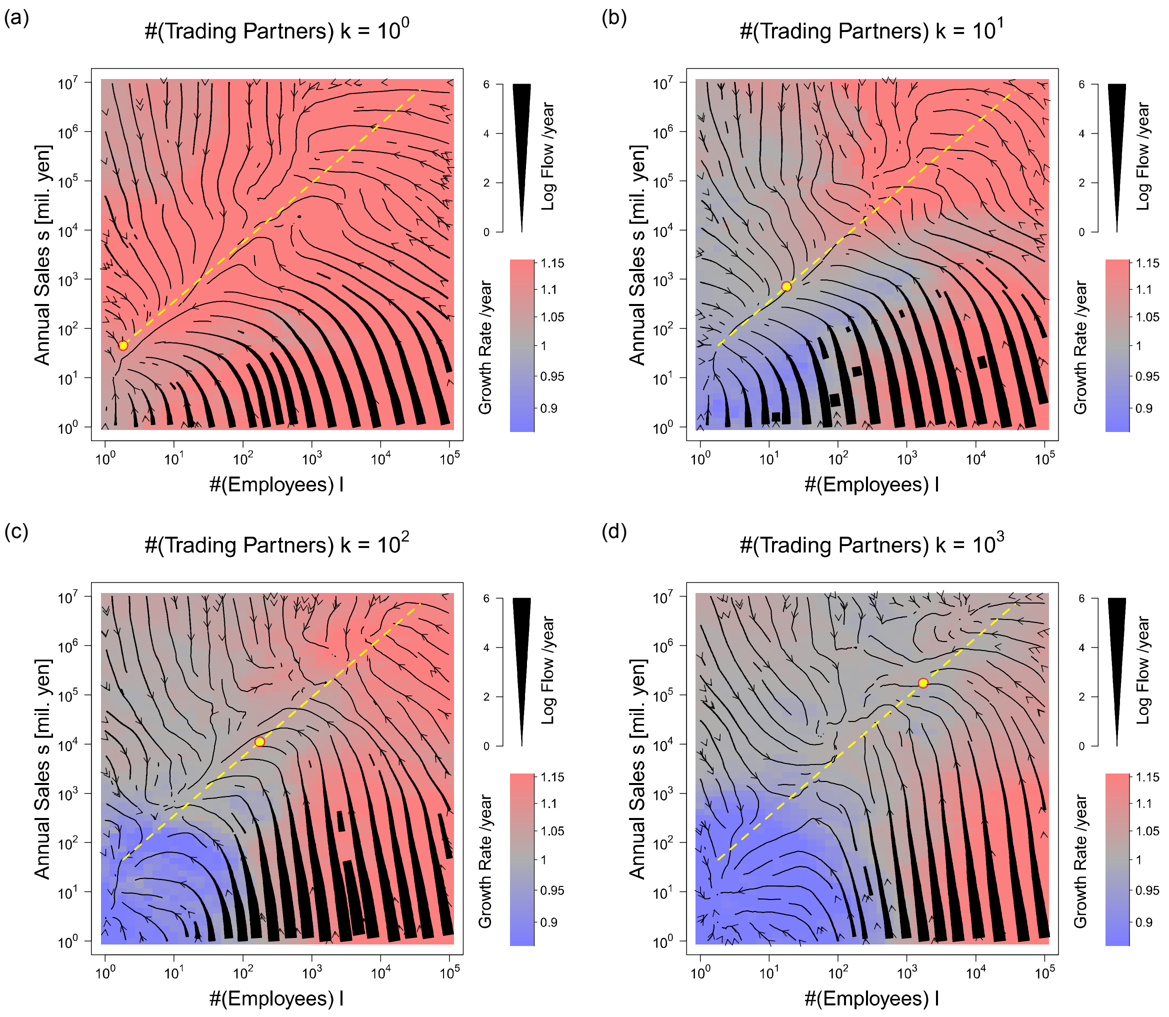


**Figure S9. Evolutionary Flow Diagram, which illustrates estimated average log-transformed growth per year in the slice of the vector space.** The direction and width of the black curves drawn indicate the velocity vector of average flow in the slicing plane. The estimated average flow orthogonal to the plane is illustrated with a background color, red, grey or blue representing plus, zero or minus growth. The yellow dashed line indicates the orthogonal projection of the scaling line to the "slicing plane" and the yellow and red point on the line represents the intersection point of the slicing plane with the scaling line. (**a–e**) The variable space is sliced by the plane of trading partners $k$ equal to 0–4 in common logarithm. (**f–j**) The variable space is sliced by the plane of employee number $l$ equal to 0–4. (**k–q**) The variable space is sliced by the plane of annual sales (in million yen) $s$ equal to 0–6. Yellow solid curves represent the intersection curves of the scaling line with the slice.

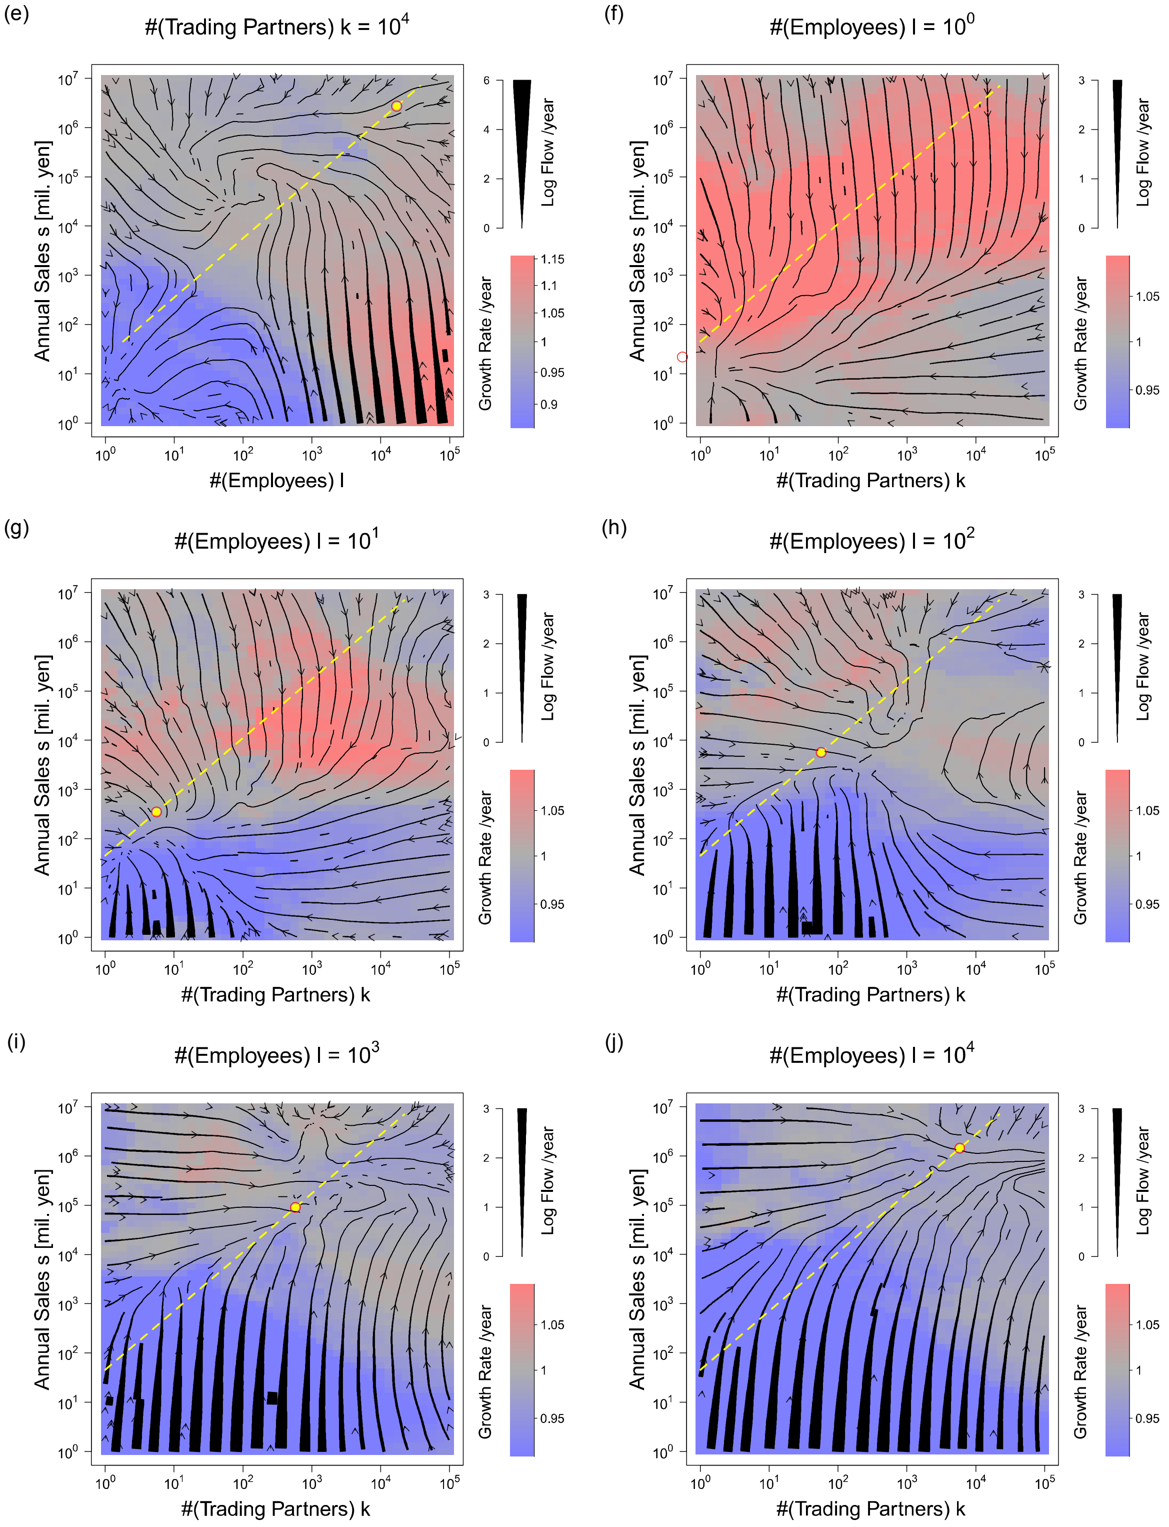


**Figure S9—Continued.**

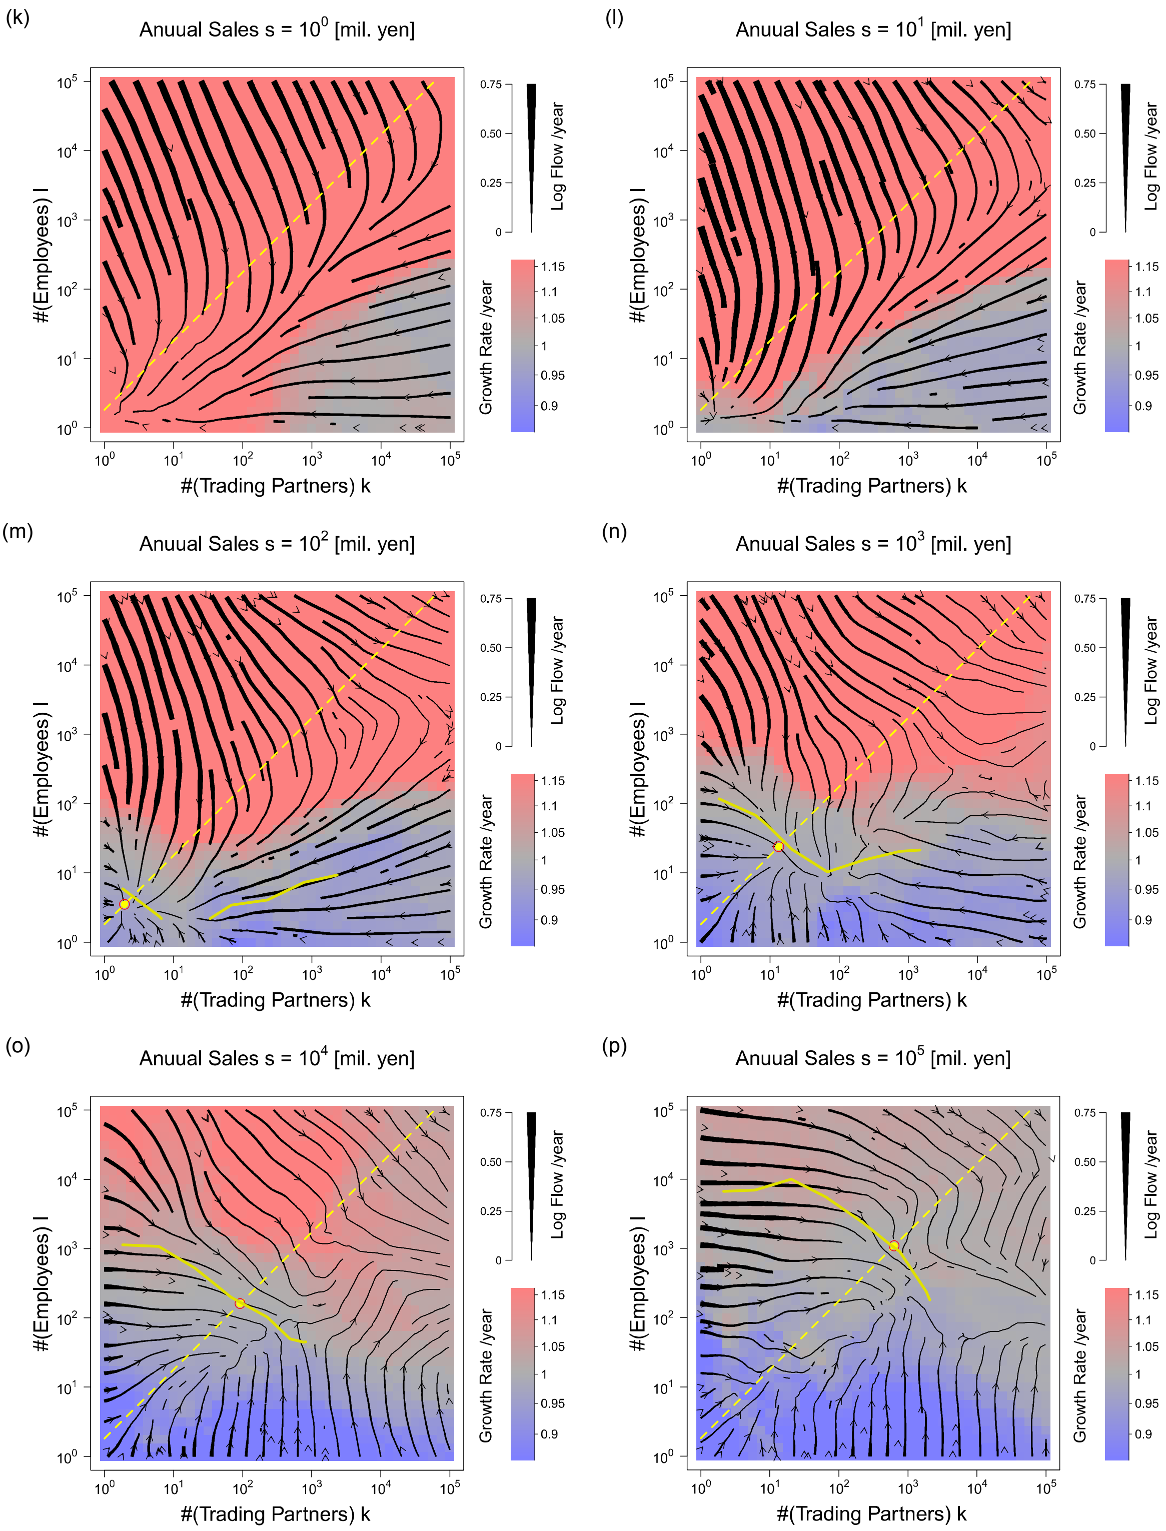


**Figure S9—Continued.**

(q)

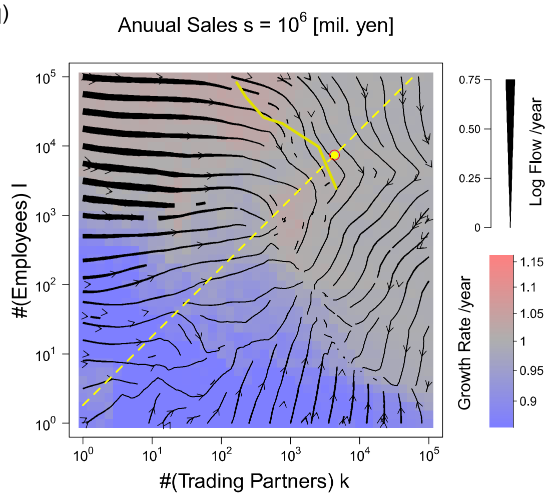


**Figure S9—Continued.**

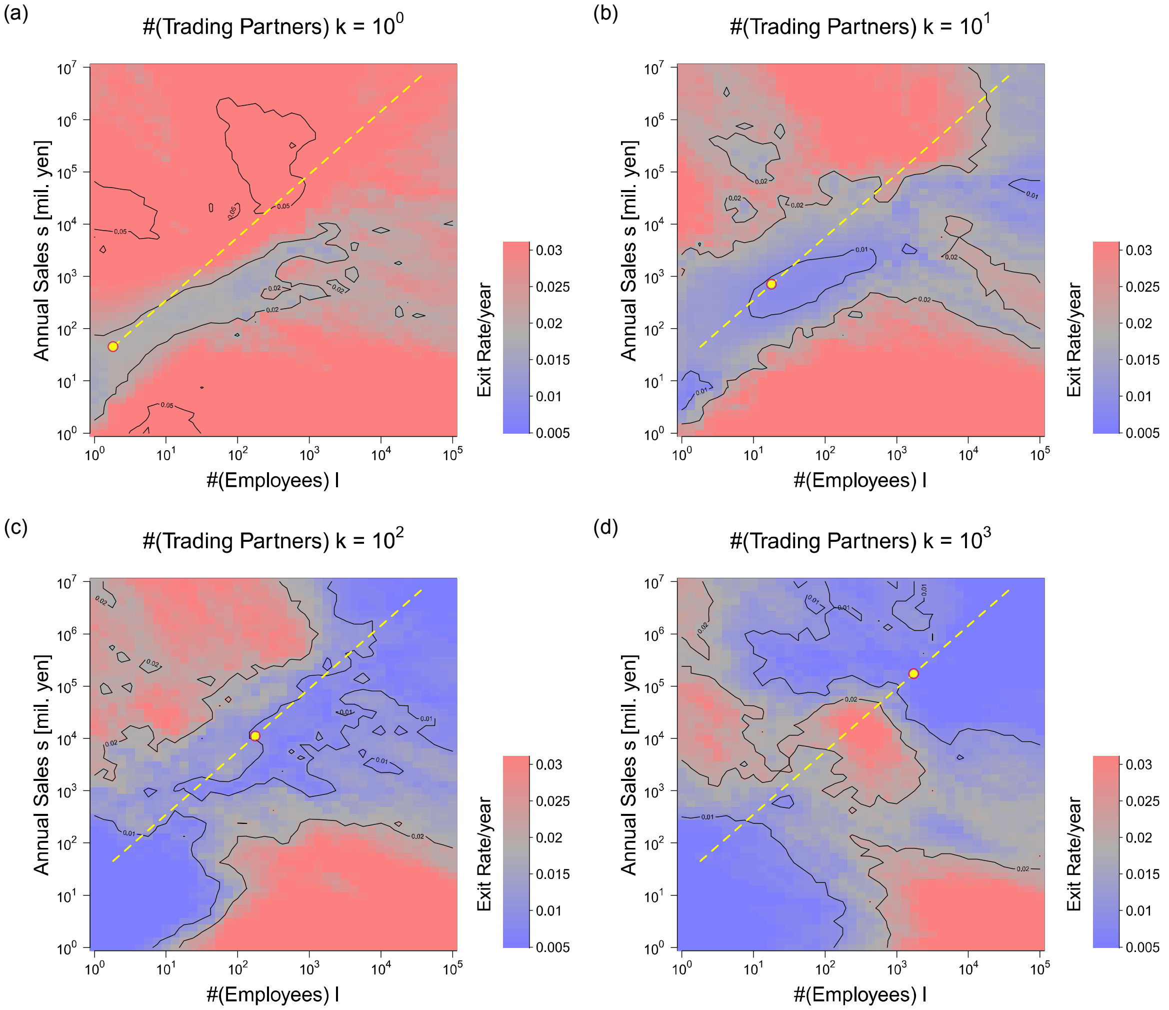


**Figure S10. Estimated exit rate per year in the slice of the log-transformed vector space.** The estimated average exit rates are illustrated by the background color, with red, grey and blue representing exit rates higher than, equal to and lower than the medium value, respectively. The yellow dashed line indicates the orthogonal projection to the "slicing line" and the yellow and red point on the line represents the intersection point of the plane with the scaling line. We add contours to show clearly the regions where exit rates are high or low. (**a–e**) The variable space is sliced by the plane of trading partners $k$ equal to 0–4 in common logarithm. (**f–j**) The variable space is sliced by the plane of employee number $l$ equal to 0–4. (**k–q**) The variable space is sliced by the plane of annual sales (in million yen) $s$ equal to 0–6. Yellow solid curves represent the intersection curves of the scaling line with the slice.

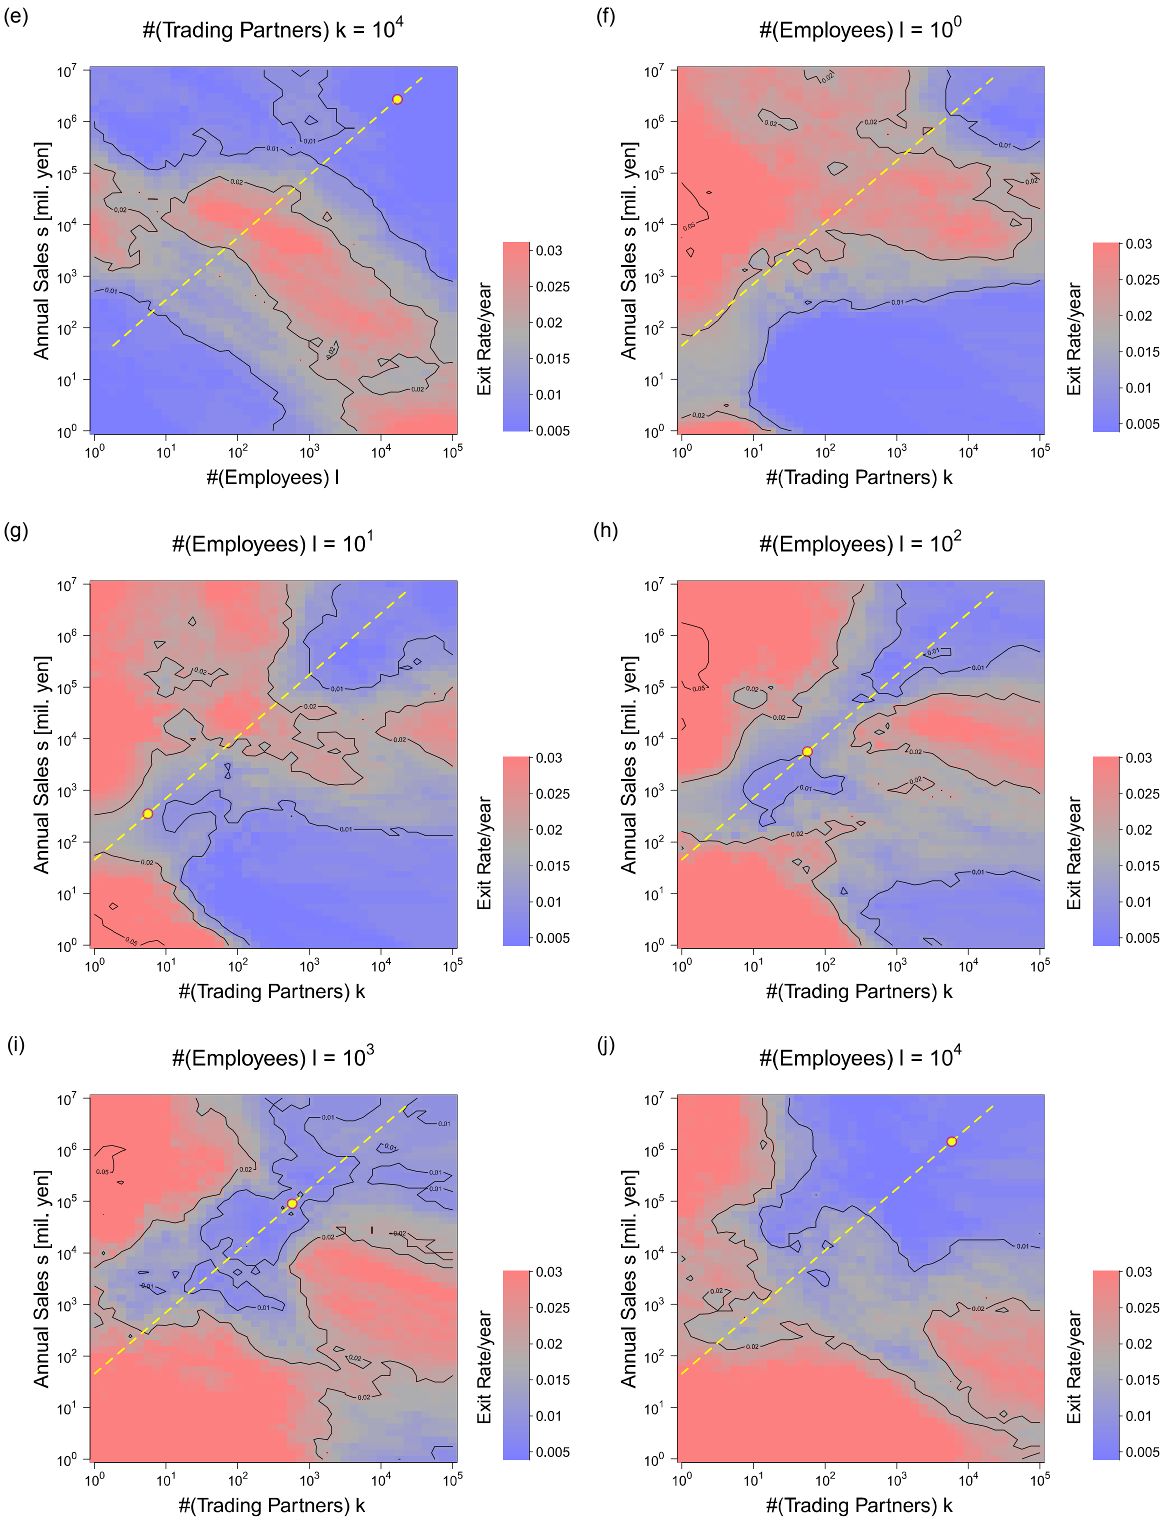


**Figure S10—Continued.**

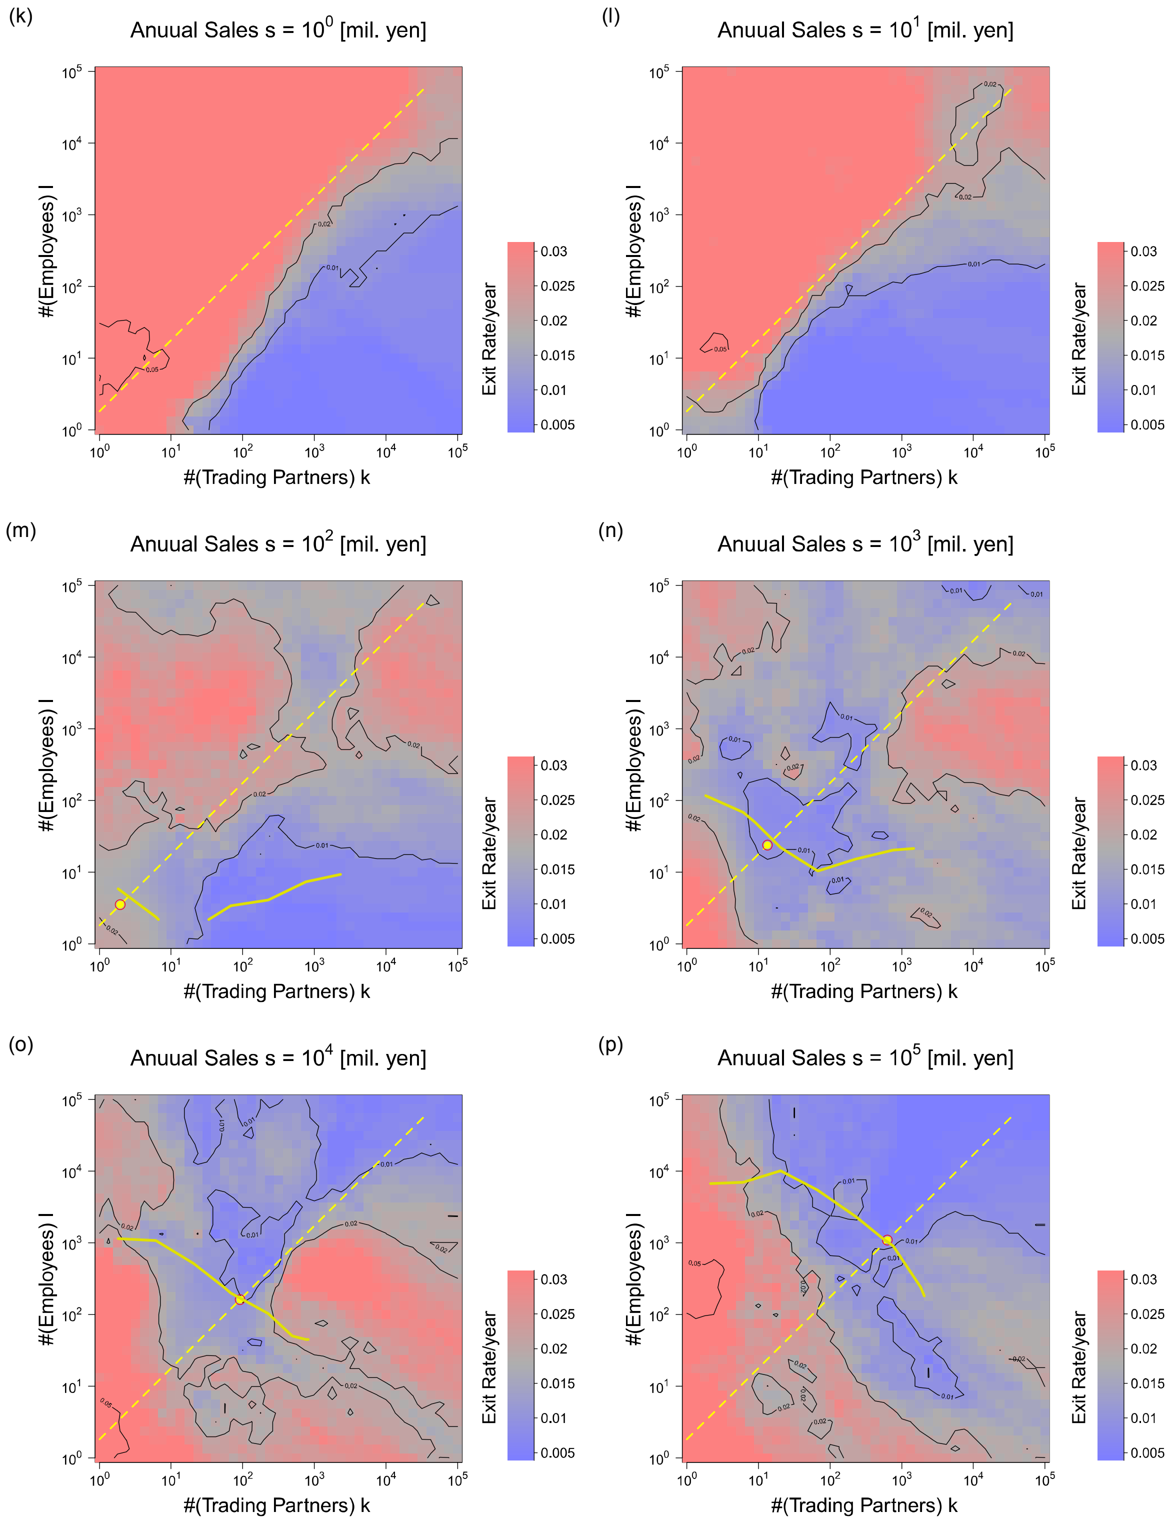


**Figure S10—Continued.**

(q)

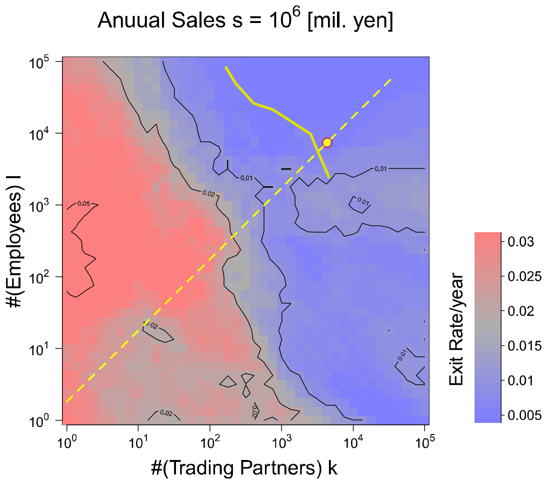


**Figure S10—Continued.**

**Table S1. Descriptive Statistics of the Final Data for Different Years.**

| Variable | Year | Mean | Standard Deviation | Minimum | 25%-quantile | Median | 75%-quantile | Maximum | Interquartile Range | Geometric Mean | Geometric Stand. Dev. |
|---|---|---|---|---|---|---|---|---|---|---|---|
| Number of Trading Partners | 1994 | 4.740 | 31.46 | 1 | 1 | 2 | 4 | 7,881 | 3 | 2.498 | 2.335 |
| | 1995 | 4.979 | 32.39 | 1 | 1 | 2 | 4 | 8,013 | 3 | 2.617 | 2.359 |
| | 1996 | 5.181 | 33.03 | 1 | 1 | 3 | 5 | 8,009 | 4 | 2.722 | 2.375 |
| | 1997 | 5.395 | 33.43 | 1 | 1 | 3 | 5 | 7,945 | 4 | 2.826 | 2.398 |
| | 1998 | 5.533 | 33.50 | 1 | 2 | 3 | 5 | 7,696 | 3 | 2.908 | 2.403 |
| | 1999 | 5.615 | 33.21 | 1 | 2 | 3 | 5 | 7,393 | 3 | 2.961 | 2.407 |
| | 2000 | 5.727 | 33.30 | 1 | 2 | 3 | 5 | 7,082 | 3 | 3.018 | 2.415 |
| | 2001 | 5.854 | 33.42 | 1 | 2 | 3 | 5 | 6,864 | 3 | 3.080 | 2.429 |
| | 2002 | 5.914 | 34.12 | 1 | 2 | 3 | 5 | 6,424 | 3 | 3.100 | 2.437 |
| | 2003 | 5.968 | 33.38 | 1 | 2 | 3 | 5 | 6,007 | 3 | 3.118 | 2.456 |
| | 2004 | 6.073 | 33.32 | 1 | 2 | 3 | 5 | 5,832 | 3 | 3.163 | 2.472 |
| | 2005 | 6.217 | 34.38 | 1 | 2 | 3 | 6 | 5,562 | 4 | 3.225 | 2.484 |
| | 2006 | 6.345 | 36.35 | 1 | 2 | 3 | 6 | 10,987 | 4 | 3.277 | 2.501 |
| | 2007 | 6.472 | 38.26 | 1 | 2 | 3 | 6 | 14,941 | 4 | 3.325 | 2.519 |
| | 2008 | 6.841 | 39.84 | 1 | 2 | 3 | 6 | 15,587 | 4 | 3.474 | 2.570 |
| | 2009 | 6.936 | 39.89 | 1 | 2 | 3 | 7 | 15,504 | 5 | 3.512 | 2.593 |
| | 2010 | 6.890 | 39.98 | 1 | 2 | 3 | 7 | 15,466 | 5 | 3.467 | 2.608 |
| | 2011 | 6.885 | 40.17 | 1 | 2 | 3 | 7 | 15,252 | 5 | 3.456 | 2.616 |
| | 2012 | 6.898 | 40.63 | 1 | 2 | 3 | 7 | 15,161 | 5 | 3.455 | 2.623 |
| | 2013 | 6.962 | 41.31 | 1 | 2 | 3 | 7 | 14,928 | 5 | 3.488 | 2.627 |
| | 2014 | 7.005 | 41.15 | 1 | 2 | 3 | 7 | 14,895 | 5 | 3.501 | 2.637 |
| | 2015 | 7.058 | 40.99 | 1 | 2 | 3 | 7 | 14,740 | 5 | 3.536 | 2.640 |

(Continued)

**Table S1. Continued.**

| Variable | Year | Mean | Standard Deviation | Minimum | 25%-quantile | Median | 75%-quantile | Maximum | Interquartile Range | Geometric Mean | Geometric Stand. Dev. |
|---|---|---|---|---|---|---|---|---|---|---|---|
| Number of Employees | 1994 | 31.48 | 424.1 | 1 | 3 | 7 | 18 | 208,028 | 15 | 8.184 | 3.787 |
| | 1995 | 30.86 | 407.2 | 1 | 3 | 7 | 18 | 191,436 | 15 | 8.059 | 3.781 |
| | 1996 | 30.21 | 396.3 | 1 | 3 | 7 | 18 | 186,706 | 15 | 7.947 | 3.763 |
| | 1997 | 29.71 | 374.0 | 1 | 3 | 7 | 17 | 161,488 | 14 | 7.830 | 3.764 |
| | 1998 | 28.97 | 360.7 | 1 | 3 | 7 | 17 | 146,744 | 14 | 7.597 | 3.763 |
| | 1999 | 27.57 | 316.5 | 1 | 3 | 6 | 15 | 77,033 | 12 | 7.235 | 3.743 |
| | 2000 | 26.86 | 311.1 | 1 | 3 | 6 | 15 | 84,242 | 12 | 7.010 | 3.741 |
| | 2001 | 25.85 | 299.1 | 1 | 3 | 6 | 15 | 91,026 | 12 | 6.764 | 3.722 |
| | 2002 | 24.78 | 287.3 | 1 | 3 | 5 | 14 | 97,474 | 11 | 6.464 | 3.705 |
| | 2003 | 24.08 | 277.4 | 1 | 2 | 5 | 13 | 100,090 | 11 | 6.253 | 3.701 |
| | 2004 | 24.18 | 380.1 | 1 | 2 | 5 | 13 | 271,368 | 11 | 6.162 | 3.717 |
| | 2005 | 24.74 | 382.2 | 1 | 2 | 5 | 13 | 261,937 | 11 | 6.162 | 3.766 |
| | 2006 | 24.51 | 357.4 | 1 | 2 | 5 | 13 | 256,572 | 11 | 6.130 | 3.759 |
| | 2007 | 25.15 | 384.4 | 1 | 2 | 5 | 13 | 254,177 | 11 | 6.111 | 3.787 |
| | 2008 | 25.14 | 335.3 | 1 | 2 | 5 | 13 | 143,276 | 11 | 6.023 | 3.791 |
| | 2009 | 24.65 | 330.7 | 1 | 2 | 5 | 12 | 140,846 | 10 | 5.842 | 3.773 |
| | 2010 | 23.80 | 325.2 | 1 | 2 | 5 | 12 | 136,906 | 10 | 5.644 | 3.745 |
| | 2011 | 23.68 | 323.9 | 1 | 2 | 5 | 11 | 139,320 | 9 | 5.549 | 3.740 |
| | 2012 | 24.02 | 366.7 | 1 | 2 | 5 | 11 | 209,000 | 9 | 5.501 | 3.752 |
| | 2013 | 23.89 | 349.4 | 1 | 2 | 5 | 11 | 200,601 | 9 | 5.489 | 3.762 |
| | 2014 | 24.06 | 354.8 | 1 | 2 | 4 | 11 | 194,688 | 9 | 5.471 | 3.772 |
| | 2015 | 24.46 | 356.7 | 1 | 2 | 5 | 12 | 193,934 | 10 | 5.516 | 3.803 |

(Continued)

**Table S1. Continued.**

| Variable | Year | Mean | Standard Deviation | Minimum | 25%-quantile | Median | 75%-quantile | Maximum | Interquartile Range | Geometric Mean | Geometric Stand. Dev. |
|---|---|---|---|---|---|---|---|---|---|---|---|
| Annual Sales [million yen] | 1994 | 2,379 | 143,058 | 1 | 70 | 180 | 480 | 39,262,034 | 410 | 198.6 | 4.587 |
| | 1995 | 2,356 | 141,562 | 1 | 70 | 180 | 469 | 39,696,346 | 399 | 195.1 | 4.601 |
| | 1996 | 2,369 | 141,412 | 1 | 70 | 178 | 470 | 39,841,681 | 400 | 194.2 | 4.636 |
| | 1997 | 2,377 | 146,488 | 1 | 70 | 173 | 464 | 55,760,824 | 394 | 191.3 | 4.694 |
| | 1998 | 2,239 | 139,637 | 1 | 62 | 160 | 426 | 56,946,664 | 364 | 176.1 | 4.707 |
| | 1999 | 2,059 | 127,448 | 1 | 58 | 145 | 390 | 48,191,575 | 332 | 161.3 | 4.685 |
| | 2000 | 2,024 | 125,415 | 1 | 54 | 137 | 370 | 46,324,909 | 316 | 153.2 | 4.734 |
| | 2001 | 1,967 | 128,025 | 1 | 50 | 128 | 350 | 48,549,384 | 300 | 143.5 | 4.799 |
| | 2002 | 1,971 | 150,814 | 1 | 45 | 118 | 321 | 67,876,272 | 276 | 132.3 | 4.825 |
| | 2003 | 2,015 | 167,481 | 1 | 43 | 110 | 309 | 75,747,636 | 266 | 125.9 | 4.878 |
| | 2004 | 1,988 | 156,492 | 1 | 42 | 109 | 304 | 71,403,288 | 262 | 124.0 | 4.940 |
| | 2005 | 1,996 | 150,736 | 1 | 41 | 108 | 306 | 74,671,935 | 265 | 123.8 | 5.002 |
| | 2006 | 2,157 | 183,258 | 1 | 40 | 107 | 308 | 106,808,600 | 268 | 123.0 | 5.079 |
| | 2007 | 2,214 | 185,985 | 1 | 40 | 104 | 305 | 105,792,700 | 265 | 121.3 | 5.161 |
| | 2008 | 2,294 | 246,066 | 1 | 39 | 100 | 300 | 181,743,800 | 261 | 114.7 | 5.277 |
| | 2009 | 2,163 | 242,882 | 1 | 32 | 90 | 260 | 177,479,800 | 228 | 99.07 | 5.371 |
| | 2010 | 2,140 | 258,782 | 1 | 30 | 80 | 237 | 175,797,700 | 207 | 89.95 | 5.394 |
| | 2011 | 2,168 | 255,034 | 1 | 30 | 80 | 230 | 174,653,200 | 200 | 87.06 | 5.475 |
| | 2012 | 2,149 | 256,620 | 1 | 29 | 80 | 230 | 175,635,300 | 201 | 86.11 | 5.517 |
| | 2013 | 2,173 | 262,035 | 1 | 29 | 79 | 224 | 176,096,136 | 195 | 85.21 | 5.528 |
| | 2014 | 2,371 | 283,726 | 1 | 29 | 80 | 231 | 176,612,700 | 202 | 86.70 | 5.668 |
| | 2015 | 2,405 | 289,929 | 1 | 29 | 80 | 235 | 177,710,700 | 206 | 87.06 | 5.696 |

*Decimal parts are rounded when the figure exceeds 4 digits.

## Supplementary References


[1] P. Cirillo and J. Hüsler, Physica A **388**, 1546 (2009).

[2] T. Ogwang, Empir. Econ. **41**, 473 (2011).

[3] B. Fix, PLoS One **12**, e0171823 (2017).

[4] M. H. R. Stanley, L. A. N. Amaral, S. V. Buldyrev, S. Havlin, H. Leschhorn, P. Maass, M. A. Salinger, and H. E. Stanley, Nature **379**, 804 (1996).

[5] G. Bottazzi and A. Secchi, RAND J. Econ. **37**, 235 (2006).

[6] H. Watanabe, H. Takayasu, and M. Takayasu, Physica A **392**, 741 (2013).

[7] A. C. Davison and D. V. Hinkley, *Bootstrap Methods and Their Application* (Cambridge University Press, Cambridge, 1997).

[8] Cabinet Office Government of Japan, (2017).

[9] Cabinet Office Government of Japan, (2017).

[10] L. A. N. Amaral, S. V Buldyrev, S. Havlin, P. Maass, M. A. Salinger, H. Eugene Stanley, and M. H. . Stanley, Physica A **244**, 1 (1997).

[11] G. De Fabritiis, F. Pammolli, and M. Riccaboni, Physica A **324**, 38 (2003).

[12] M. Takayasu, H. Watanabe, and H. Takayasu, J. Stat. Phys. **155**, 47 (2014).

[13] A. Ishikawa, S. Fujimoto, T. Mizuno, and T. Watanabe, in *Proc. Asia-Pacific Econophysics Conf. 2016 — Big Data Anal. Model. Towar. Super Smart Soc. —*, edited by M. Takayasu (Journal of the Physical Society of Japan, Tokyo, 2017), p. 11005.

[14] G. Turk and D. Banks, in *Proc. 23rd Annu. Conf. Comput. Graph. Interact. Tech. - SIGGRAPH '96* (ACM Press, New York, New York, USA, 1996), pp. 453–460.
